# Supplementary material for: Dynamical Landscape and Multistability of a Climate Model
Source: arXiv:2010.10374 source file (2021-01-08)
Supplement: Supplementary file 1 [file supplamentary_material.tex]

%% Author_tex.tex
%% V1.0
%% 2012/13/12
%% developed by Techset
%%
%% This file describes the coding for rsproca.cls

\documentclass[openacc]{rsproca_new}%%%%where rsproca is the template name

%%%% *** Do not adjust lengths that control margins, column widths, etc. ***

\usepackage{graphicx,color}
\usepackage{dcolumn}% Align table columns on decimal point
\usepackage{url} %this package should fix any errors with URLs in refs.
\usepackage{amsmath,amsfonts,amsthm,bm,amssymb} 
\usepackage{booktabs}
%\graphicspath{ {SM_plots/} }
\usepackage{hyperref,comment}
\usepackage{float}
\usepackage{soul}
\usepackage{natbib}
\setcitestyle{numbers,sort&compress}

    % VL
    % GM
    % TG
    % AL

%%%%%%%%%%% Defining Enunciations  %%%%%%%%%%%

%%%%%%%%%%%%%%%%%%%%%%%%%%%%%%%%%%%%%%%%%%%%%%%

\begin{document}

%%%% Article title to be placed here
\title{Dynamical Landscape and Multistability of a Climate Model}

\author{%%%% Author details
Georgios Margazoglou$^{1,2}$, Tobias Grafke$^{3}$, Alessandro Laio$^{4}$ and Valerio Lucarini$^{1,2}$}

%%%%%%%%% Insert author address here
\address{$^{1}$Department of Mathematics and Statistics, University of Reading, Reading, United Kingdom\\
$^{2}$Centre for the Mathematics of Planet Earth, University of Reading, Reading, United Kingdom\\
$^{3}$Mathematics Institute, University of Warwick, United Kingdom\\
$^{4}$International School for Advanced Studies (SISSA), Trieste, Italy}

%%%% Subject entries to be placed here %%%%
\subject{Climatology, Statistical Physics, Artificial Intelligence}

%%%% Keyword entries to be placed here %%%%
\keywords{Climate modelling, multistability, quasipotential theory, nonequilibrium systems, data-driven methods, manifold learning}

%%%% Insert corresponding author and its email address}
\corres{Valerio Lucarini\\
\email{v.lucarini@reading.ac.uk}}

%%%% Abstract text to be placed here %%%%%%%%%%%%
\begin{abstract}
We apply two independent data analysis methodologies to locate stable climate states in an intermediate complexity climate model. First, drawing from the theory of quasipotentials, and viewing the state space as an energy landscape with valleys and mountain ridges, we infer the relative likelihood of the identified multistable climate states, and investigate the most likely transition trajectories as well as the expected transition times between them. Second, harnessing techniques from data science, specifically manifold learning, we characterize  the data landscape of the simulation output to find climate states and basin boundaries within a fully agnostic and unsupervised framework. Both approaches show remarkable agreement, and reveal, apart from the well known warm and snowball earth states, a third intermediate stable state in one of the two climate models we consider. The combination of our approaches allows to identify how the negative feedback of ocean heat transport and entropy production via the hydrological cycle drastically change the topography of the dynamical landscape of Earth's climate.
\end{abstract}
%%%%%%%%%%%%%%%%%%%%%%%%%%%

%\maketitle

{\noindent \Large \color{jobcolor}
	\begin{center}
\underline{Supplementary Material} for ``Dynamical Landscape and Multistability of a Climate Model''
	\end{center} }
\begin{center}
Georgios Margazoglou$^{1,2}$, Tobias Grafke$^{3}$, Alessandro Laio$^{4}$ and Valerio Lucarini$^{1,2}$
\end{center}
$^{1}$Department of Mathematics and Statistics, University of Reading, Reading, United Kingdom\\
$^{2}$Centre for the Mathematics of Planet Earth, University of Reading, Reading, United Kingdom\\
$^{3}$Mathematics Institute, University of Warwick, United Kingdom\\
$^{4}$International School for Advanced Studies (SISSA), Trieste, Italy
\vspace{1cm}

In the following we provide supporting material and information to the main paper. We further provide a set of animations that illustrate the real-time evolution of the system when transitions among the basins of attraction occur.

\section{Methods for Estimating the Transition Paths}\label{sec:paths}
The estimate of the average transitions path is performed as follows. 
\begin{enumerate}
	\item We first define a line  -- thin dashed black line in Fig.~\ref{fig:ocdiff_1_phsp}~-- that clearly separates between the two metastable states;
	\item We check whether a portion of the orbit, coming from a neighbourhood of the $\Omega_1$ attractor, crosses the  line, and eventually enters the neighbourhood of the attractor $\Omega_2$;
	\item If so, and the trajectory remained near $\Omega_1$  for at least $y$ years and then remains for $Y$ years near $\Omega_2$, we  store the $y+Y$ years long trajectory;
	\item We perform a time average of the final set of trajectories. 
\end{enumerate}

\begin{figure}[h!]
	\centering
	\includegraphics[width=.49\linewidth]{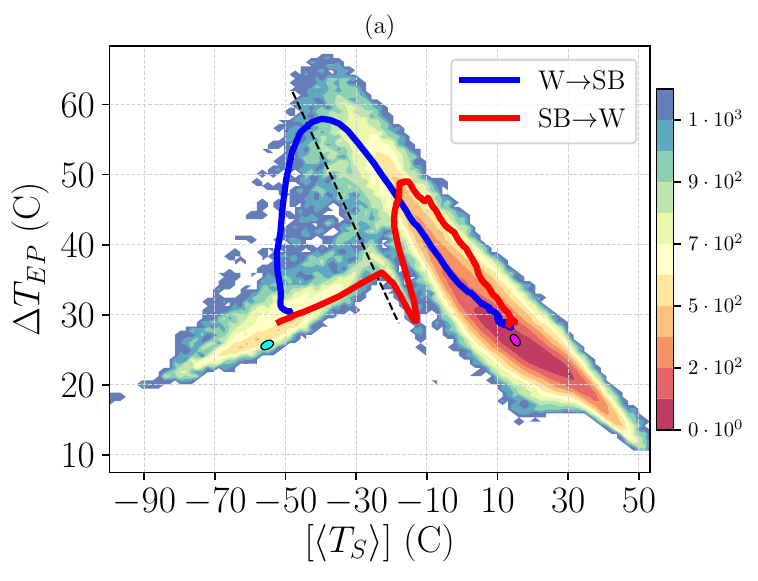} 
	\includegraphics[width=.49\linewidth]{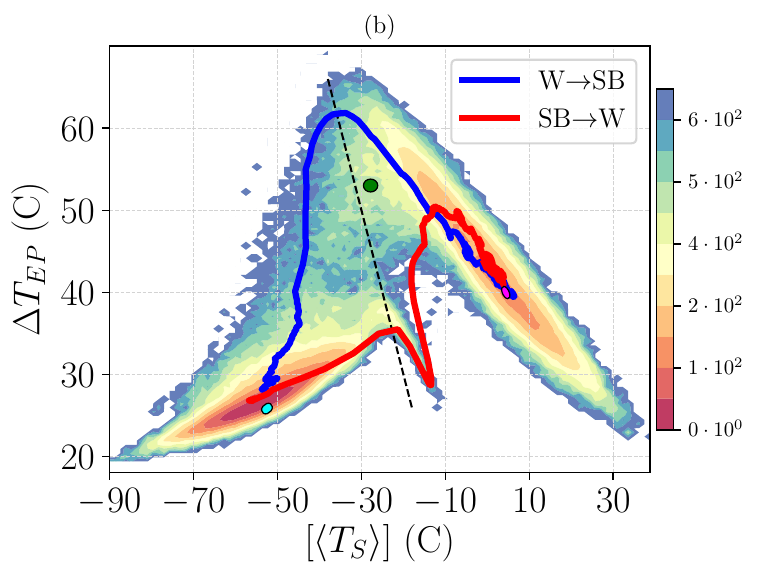} 
	\caption{ (a) Projection of the quasipotential on the reduced phase space spanned by the 30-day averaged global temperature versus 30-day averaged Equator to pole temperature difference for setup A and $\sigma=18\%$, shifted so that the global minimum is set to 0. (b) same as in (a) for setup B and $\sigma=12\%$. The blue and red lines correspond to the averaged transition paths  for the W$\rightarrow$SB and SB$\rightarrow$W transitions. These trajectories follow different escape and relaxation paths, within each basin of attraction. The colored ellipses indicate the location of the deterministic attractors corresponding to SB state (cyan), and W state (magenta). }
	\label{fig:ocdiff_1_phsp} 
\end{figure}

To improve our estimate, we combine statistics from the simulations performed with the three smallest noise intensities $\%\sigma$, obtaining a set of roughly 100 $y+Y$ years long trajectories with the properties above. Here, for setup A it holds $y+Y=2+14=16 \,yrs$ for $SB\rightarrow W$ and $y+Y=14+2=16\,yrs$ for $W\rightarrow SB$. For setup B it holds $y+Y=4+36=40 \,yrs$ for $SB\rightarrow W$ and $y+Y=40+10=50\,yrs$ for $W\rightarrow SB$. Note that the results are robust both with respect to small changes in the choices of $y$, $Y$ and of the geometry of the line used as a criterion for separating the two metastable states. 

\begin{figure*}[t]
	\centering
	\includegraphics[width=.32\linewidth]{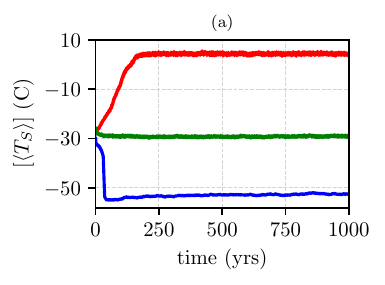}
	\includegraphics[width=.32\linewidth]{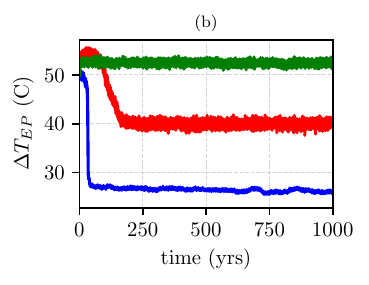} 
	\includegraphics[width=.32\linewidth]{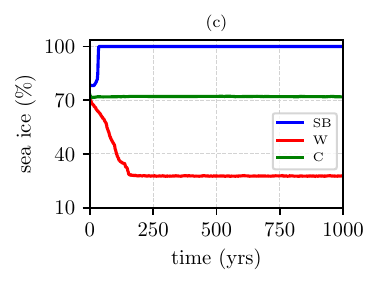}		
	\caption{Relaxation trajectories evolved in time as a function of 30-day averaged (a)  global surface temperature (b) Equator to pole temperature difference and (c) sea ice percentage, using setup B, which clearly allows for the existence of three metastable climate states.}
	\label{fig:ocdiff_0_time} 
\end{figure*}

\section{Relaxation trajectories}\label{sec:relaxation}

Figure~\ref{fig:ocdiff_0_time} provides evidence for three stable climatic states, whose basin features are reported in Table~I of the main paper. It shows the time evolution of $[\langle T_S\rangle]$, $\Delta T_{EP}$, and sea ice percentage for three trajectories initialized in an unstable region of the phase space for setup B and undergoing a deterministic evolution with a constant value for $S^* = 1365 \, \textrm{W}/\textrm{m}^2$, i.e. $\sigma=0\%$. Accordingly, Fig.~\ref{fig:setup_B_relx} shows the first 200 years of evolution of corresponding runs of Fig.~\ref{fig:ocdiff_0_time} (a-b) in the reduced phase space projection ($[\langle T_S\rangle]$, $\Delta T_{EP}$) of the invariant measure.

\begin{figure}[h]
	\centering
	\includegraphics[width=0.6\linewidth]{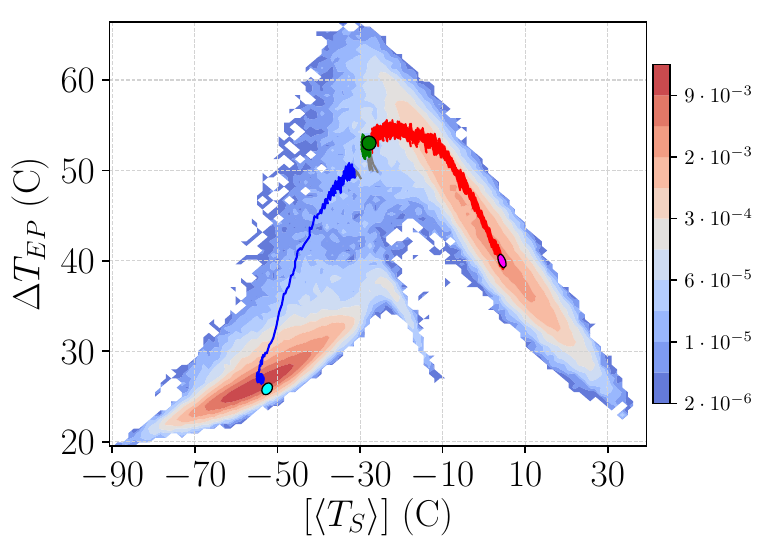}
	\caption{ The first 200 years of the relaxation trajectories of Fig.~\ref{fig:ocdiff_0_time}(a-b) in the reduced phase space projection ($[\langle T_S\rangle]$, $\Delta T_{EP}$) of the invariant measure.	}
	\label{fig:setup_B_relx} 
\end{figure}

\section{Animations}\label{sec:Animations}
We present here a series of animations that illustrate the real time  dynamics of the climate model subjected to random yearly fluctuations of the solar constant $S^*$. To convey the dramatic implications of the global transitions taking place, we further present the corresponding daily evolution of four observables.

In the following, we focus in the cases where the system exhibits a noise induced transition among its basins of attraction. The layout of the animations is the same for consistency, and the frequency is 30 frames per second (fps), to match one month per second. The left part of the animations involves the projection of the quasipotential, shifted so that the global minimum is set to 0, on the reduced phase space spanned by the 30-day averaged global temperature $[\langle T_S\rangle]$, versus 30-day averaged Equator to pole temperature difference $\Delta T_{EP}$ for either setups (e.g. see Fig.4(b) of the paper). On top of this projection, the averaged transition path is overlaid following the steps described in Sec.~\ref{sec:paths}. The interesting viewpoint is the real-time trajectory of the system in the $([\langle T_S\rangle],\Delta T_{EP})$ projected space, which is shown via the ``snake-like'' moving black line of 90-days long duration. Meanwhile, the box in the top right corner contains the month/year time-stamp together with the value of the solar constant for the particular year. 

%Notice that typically when $S^* < S^*_0 (1 - 2\sigma)$ the system is triggered towards a transition to the SB basin of attraction, while when $S^* > S^*_0 (1 + 2\sigma)$ towards the W basin of attraction, where $S^*_0 = 1365$ W/m$^2$. 
For the cases considered, unless otherwise stated, the real-time evolution is taken from the dataset with $\sigma=20\%$ for setup A and $\sigma=16\%$ for setup B \cite{datapaper}. Furthermore, as discussed in the paper, the transitions occur via two different channels indicating the existence of a current, which is a signature of nonequilibrium dynamics. 

The right part of the animations gives an account of the corresponding temporal evolution of the distribution on Earth of four relevant climatic observables; namely, the surface temperature, the wind speed at 300 hPa, the Geopotential height at 500 hPa, and the sea ice cover. As the frequency is again 30 fps, slower playback speeds would help the interested viewer to observe finer details, if necessary. When contours are used, the colormap is adjusted to effectively show all the range of values that the system exhibits during its transition. Note that the choice of the particular observables also serves the purpose of showing the different and vast timescales within the system, with the winds having timescales of days, the Geopotential of weeks, the surface temperature of months and the sea-ice coverage of years. 

Each animation is introduced via a snapshot below, which can be watched by clicking on the relevant link in the caption. 

As discussed in the main paper, the key message of the following animations is that the forward and the corresponding backwards transition between two basins of attraction follow a different path in the phase space. This is a signature of enhanced nonequilibrium conditions, that can be attributed to the presence of an active hydrological cycle in the model. Furthermore, it also suggest a different route towards the thawing and freezing of the planet.

\subsection{Setup A}
For setup A we present two movies that portray the transition from the SB to the W state (Fig. \ref{fig:setup_A_SBW}-left) and from the W to the SB state (Fig. \ref{fig:setup_A_SBW}-right). The mean escape paths are included as a red (blue) line towards the W (SB) attractor.
\begin{figure}[!h]
	\centering
	\includegraphics[width=0.49\linewidth]{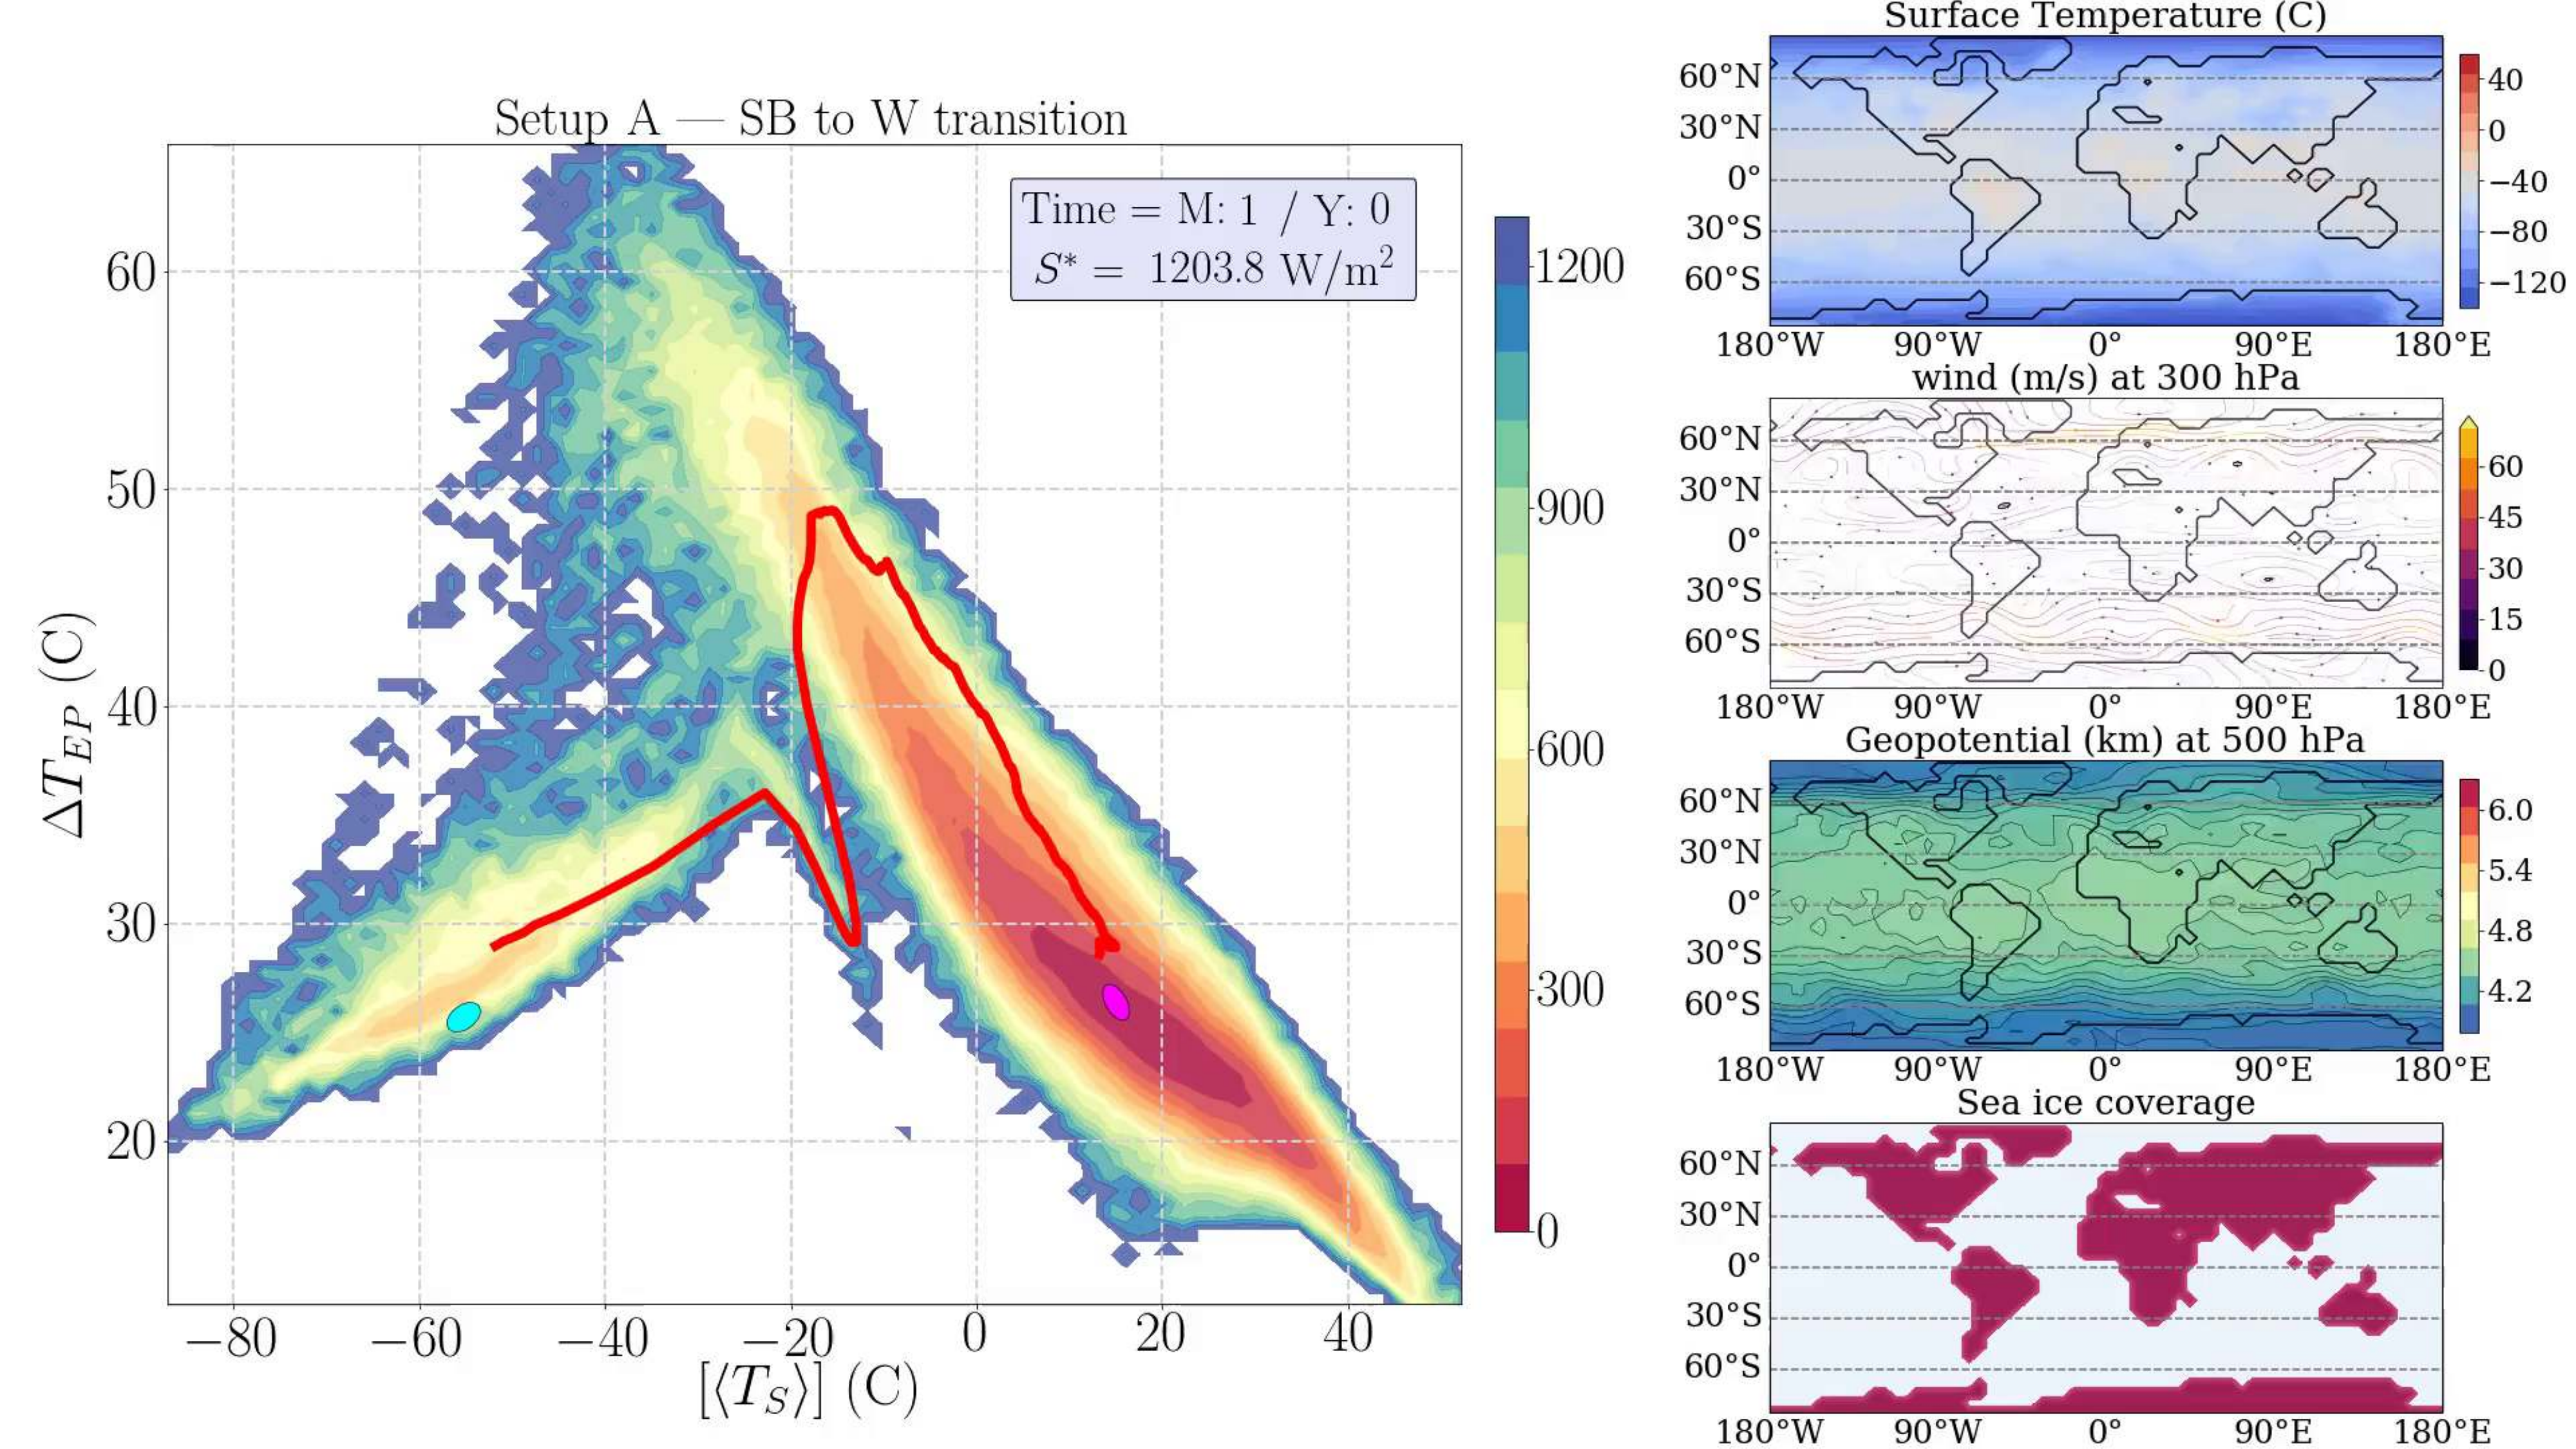}
	\includegraphics[width=0.49\linewidth]{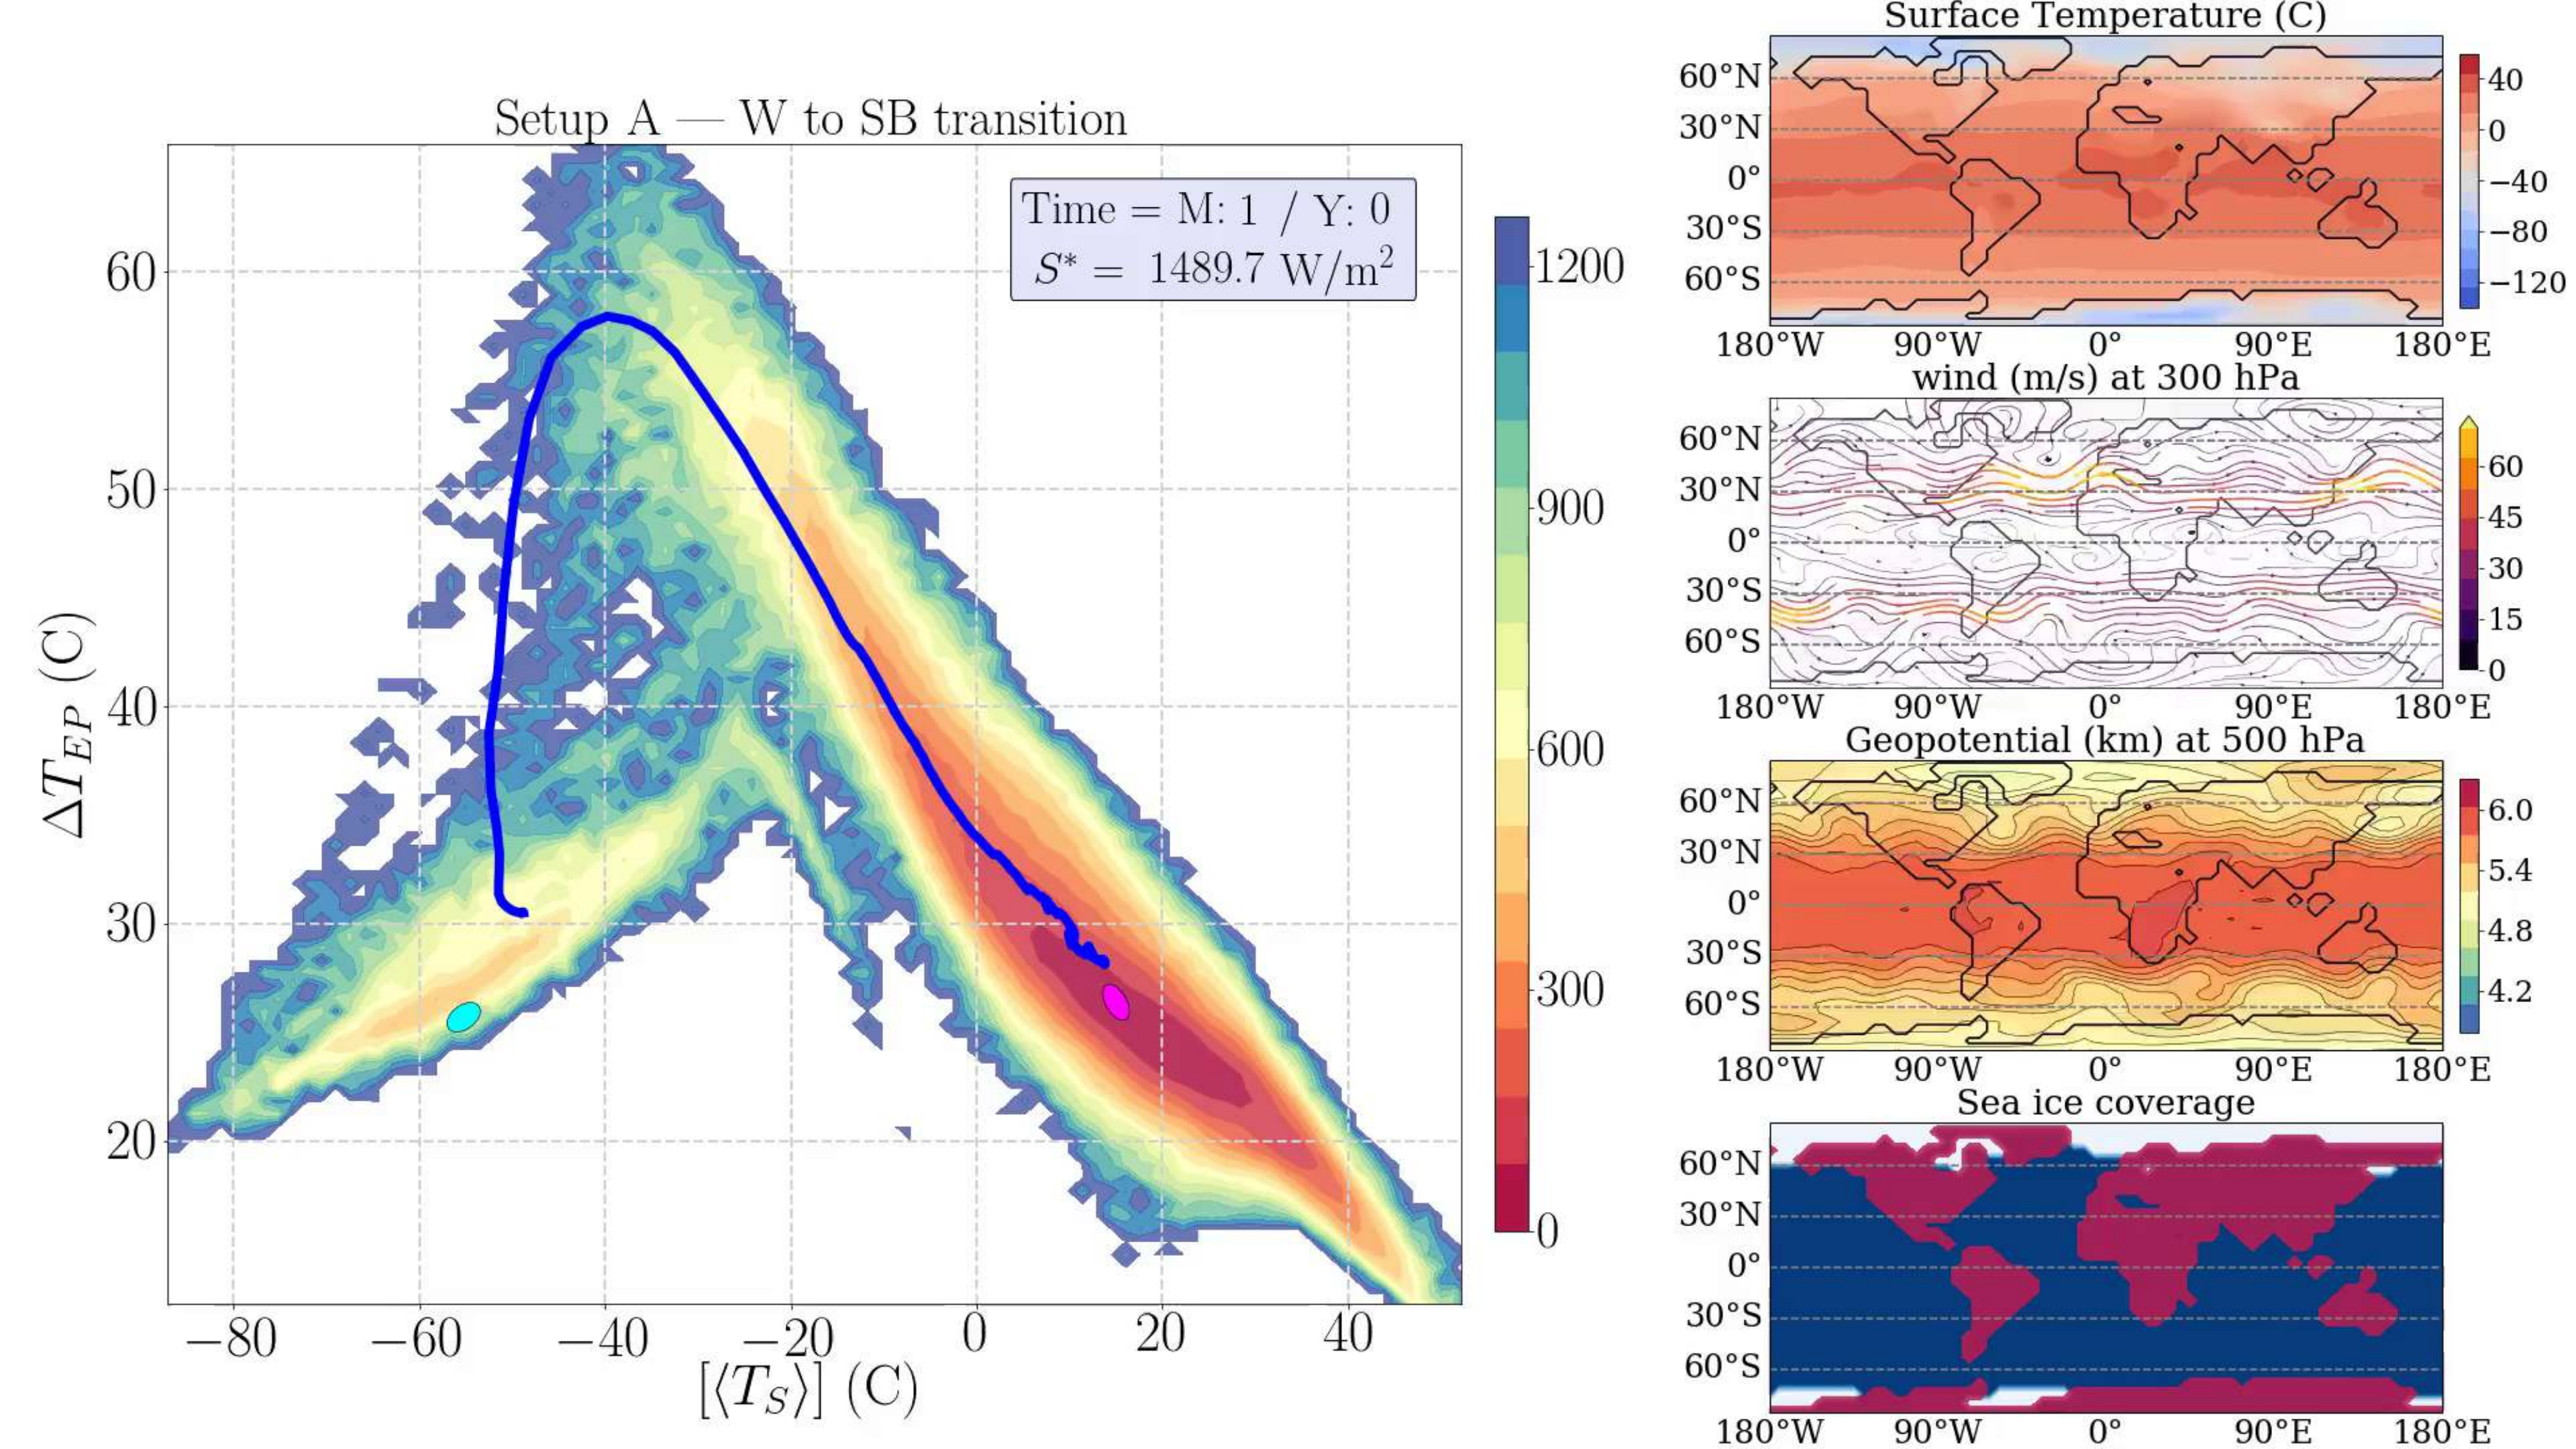}
	\caption{ Setup A: (left) Snowball to Warm transition.   \href{https://youtu.be/KJap8ifAjT4}{Click for video}. (right) Warm to Snowball transition.   \href{https://youtu.be/w8wBDhlNJc4}{Click for video}}
	\label{fig:setup_A_SBW} 
\end{figure}

\subsection{Setup B}

For setup B we present a more extended set of movies, in order to better capture the higher complexity of the dynamical landscape of this version of the model. Figures \ref{fig:setup_B_SBW}-left and \ref{fig:setup_B_SBW}-right give access to the movies that portray the direct transition from the SB to the W state and from the W to the SB state, respectively. Instead, from Figs. \ref{fig:setup_B_SBCW}-right and \ref{fig:setup_B_SBCW}-left we can access the movies portraying a transition from the SB to the W state and from the W to the SB state, respectively, that feature the C state as intermediate step. The mean direct escape paths are included as a red (blue) line towards the W (SB) attractor.

\begin{figure}[!h]
	\centering
	\includegraphics[width=0.49\linewidth]{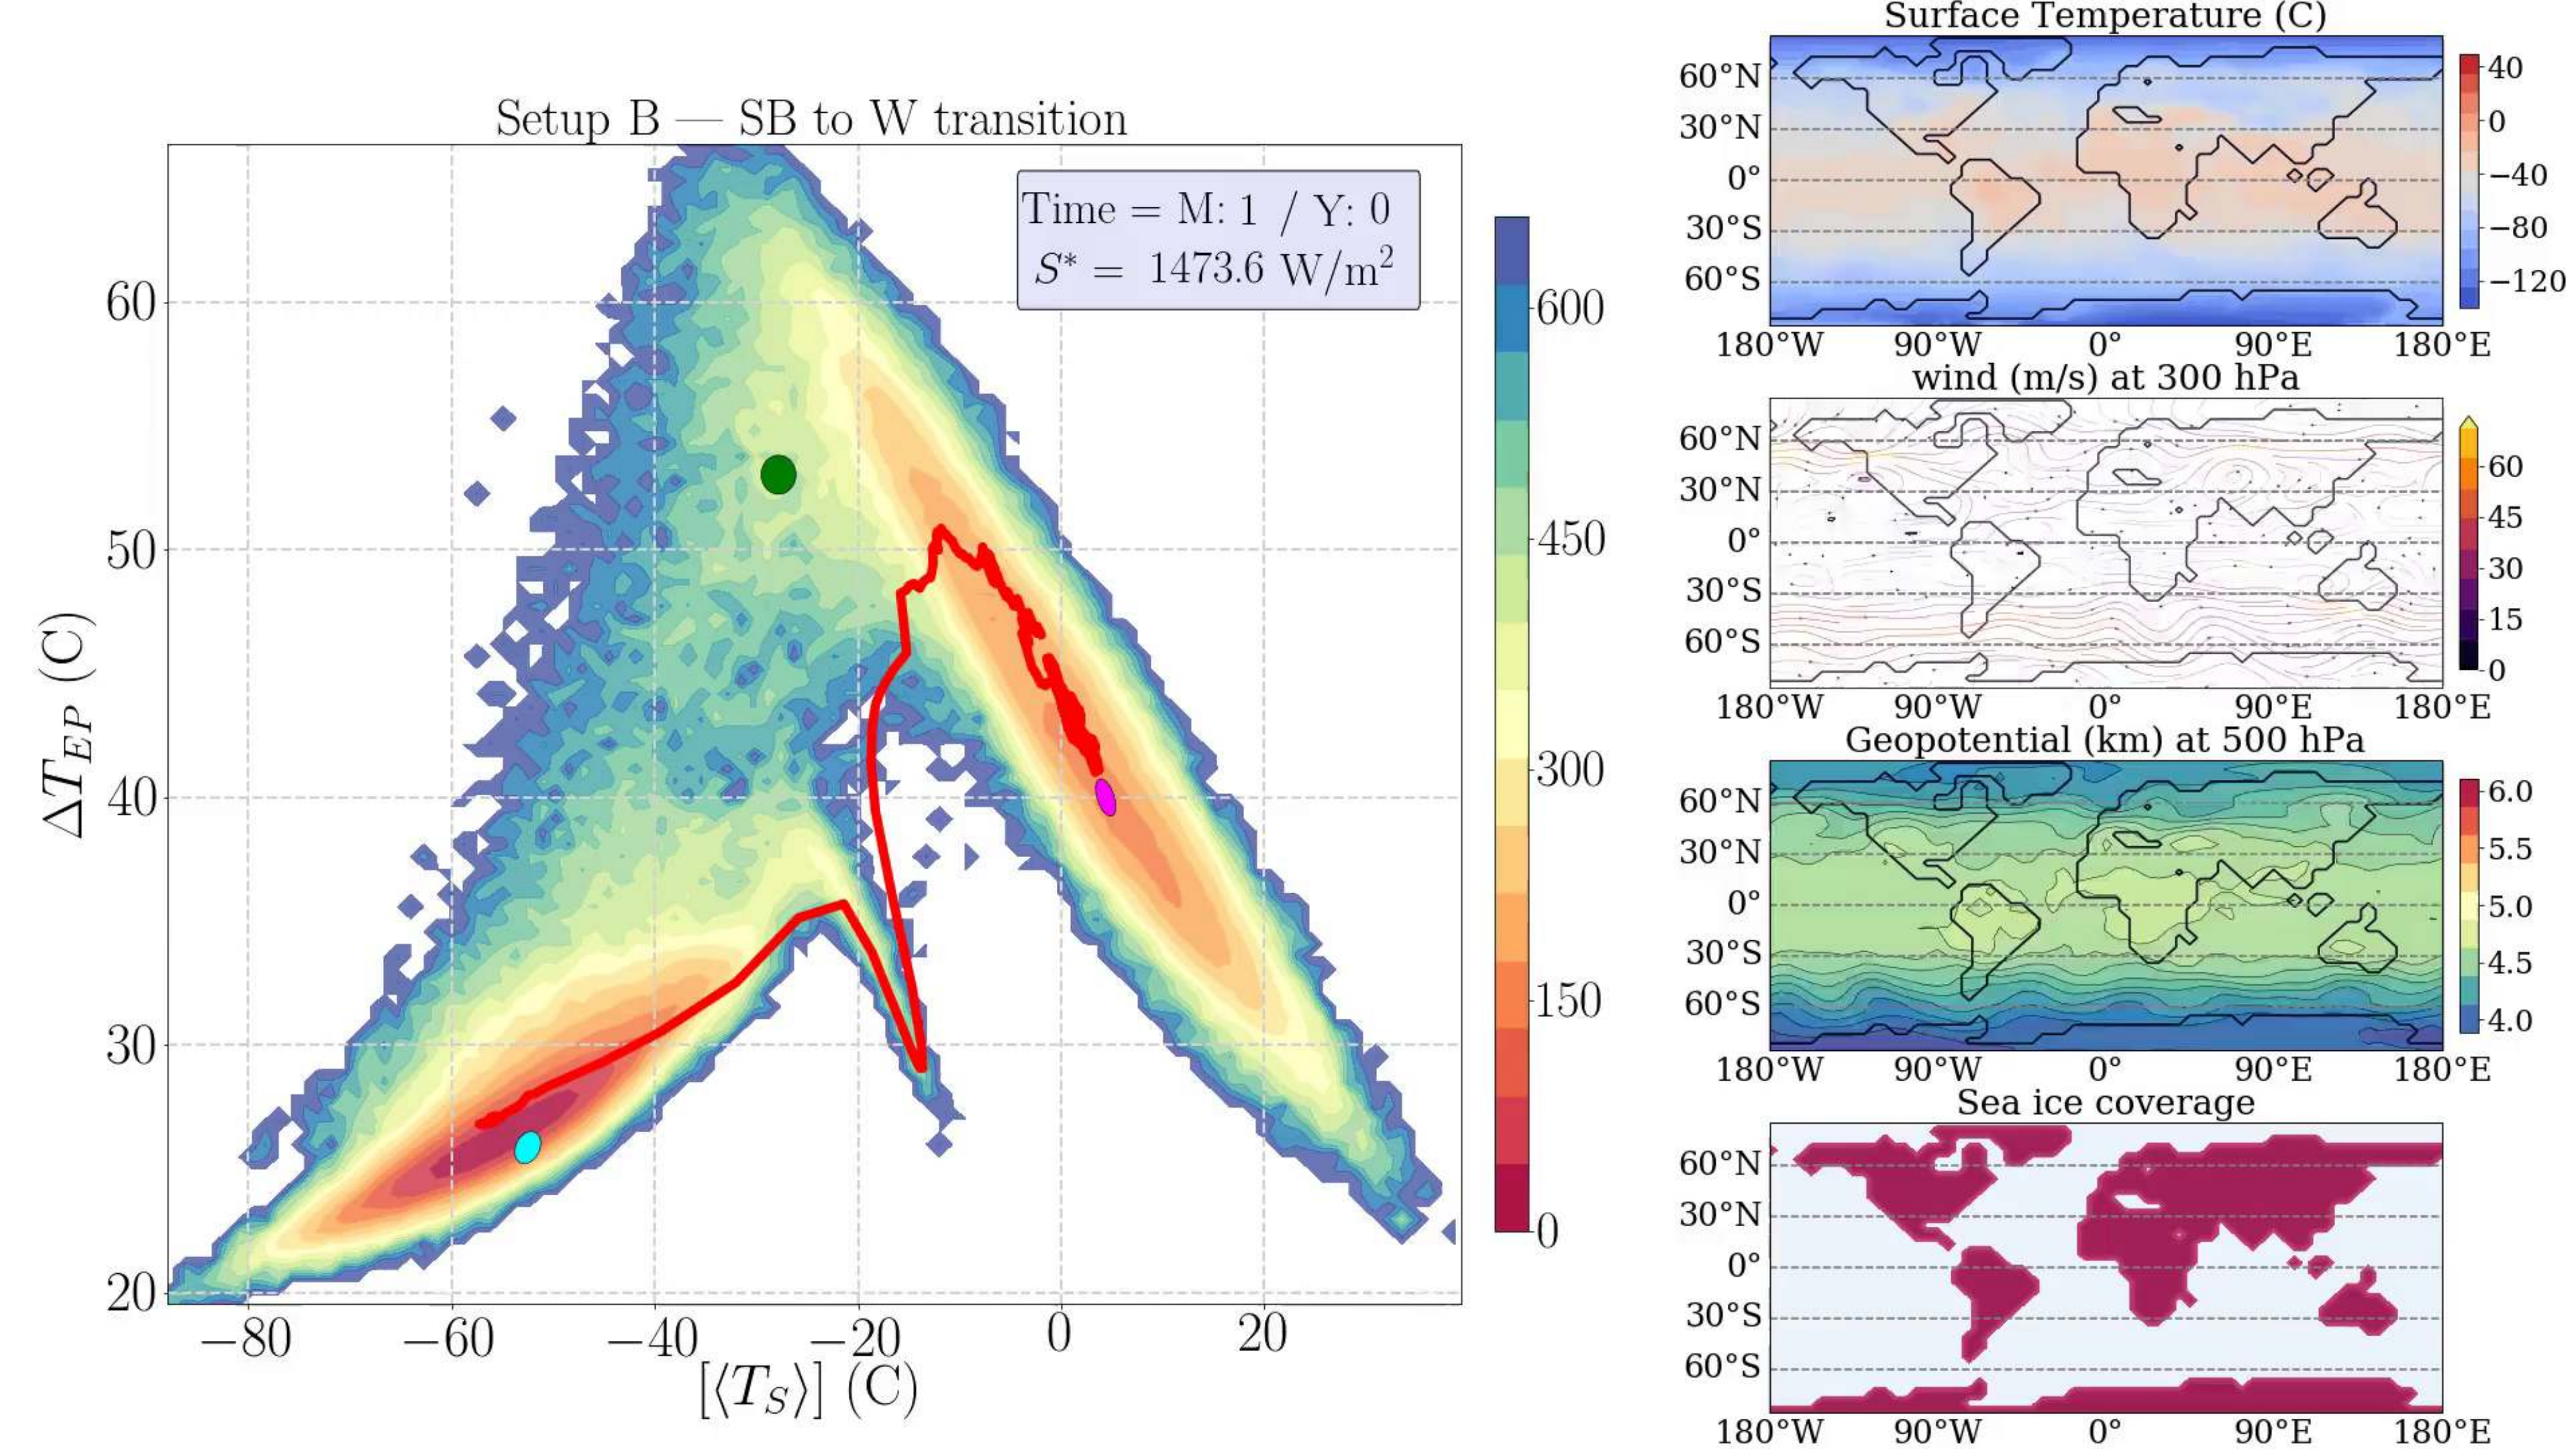}
	\includegraphics[width=0.49\linewidth]{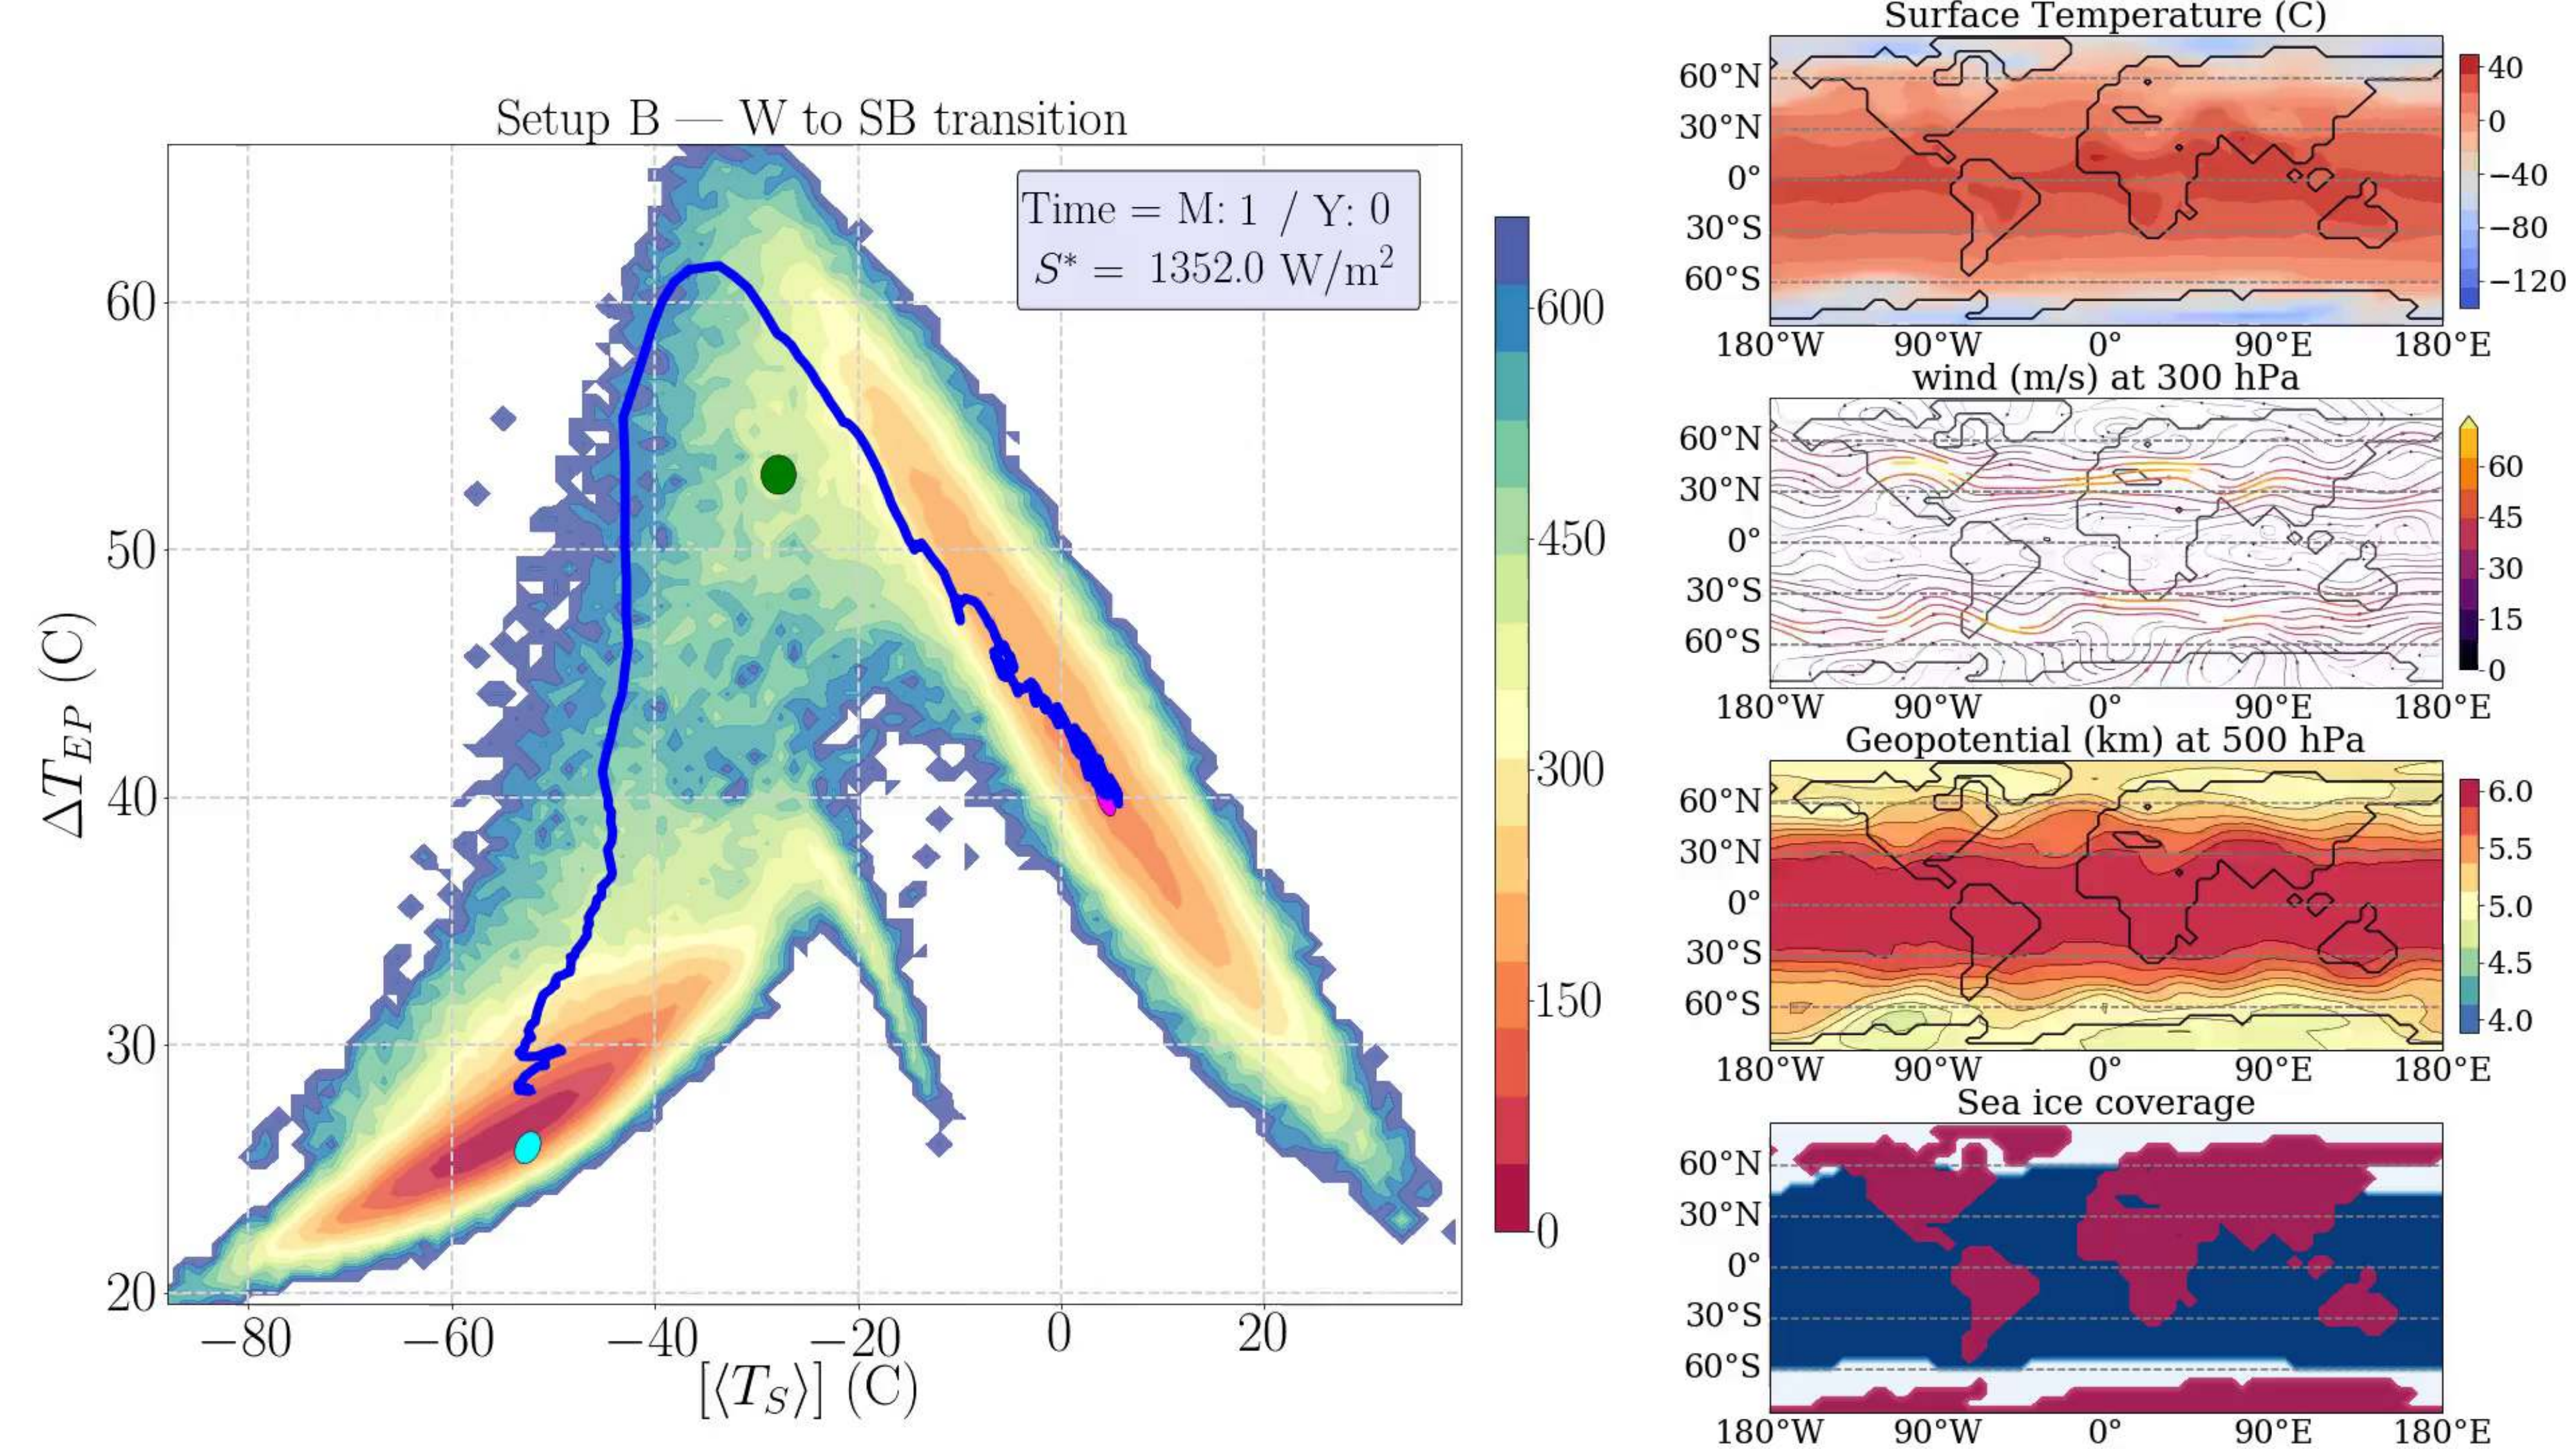}
	\caption{ Setup B: (left) Snowball to Warm transition.   \href{https://youtu.be/3vyuflCnQeE}{Click for video}. (right) Warm to Snowball transition.   \href{https://youtu.be/25DX8Isb0EM}{Click for video}}
	\label{fig:setup_B_SBW} 
\end{figure}

\begin{figure}[!h]
	\centering
	\includegraphics[width=0.49\linewidth]{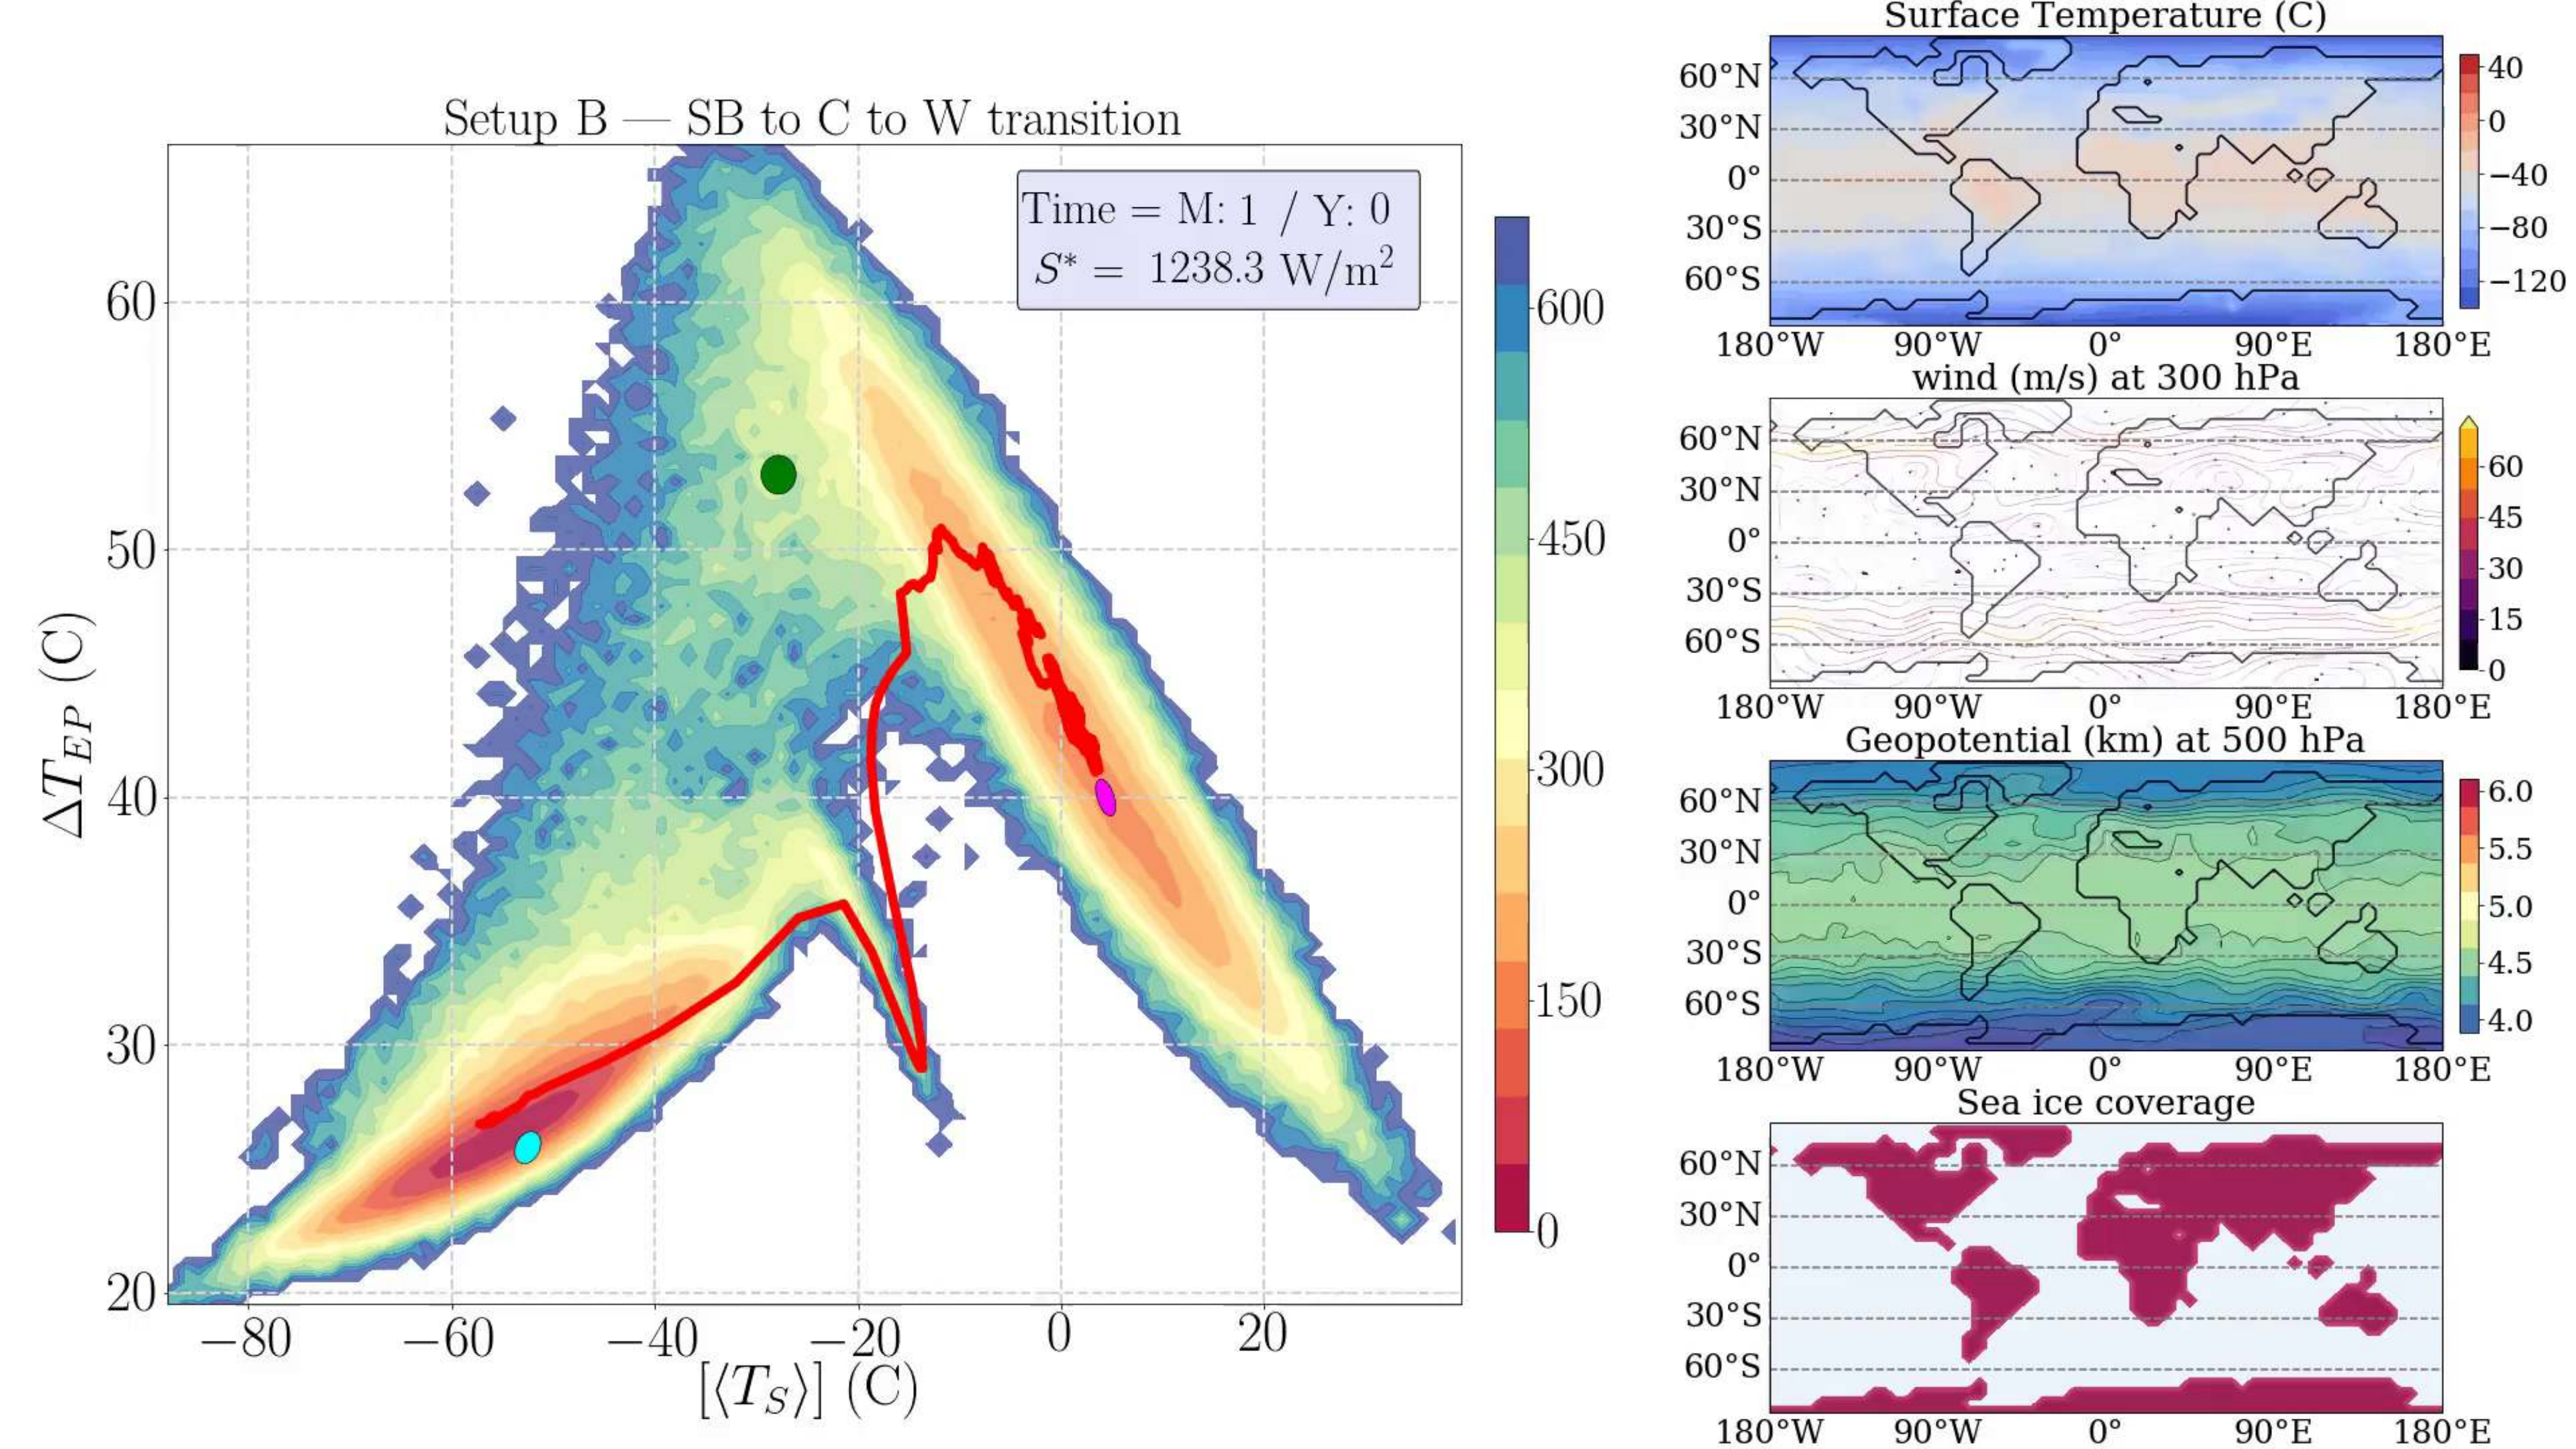}
	\includegraphics[width=0.49\linewidth]{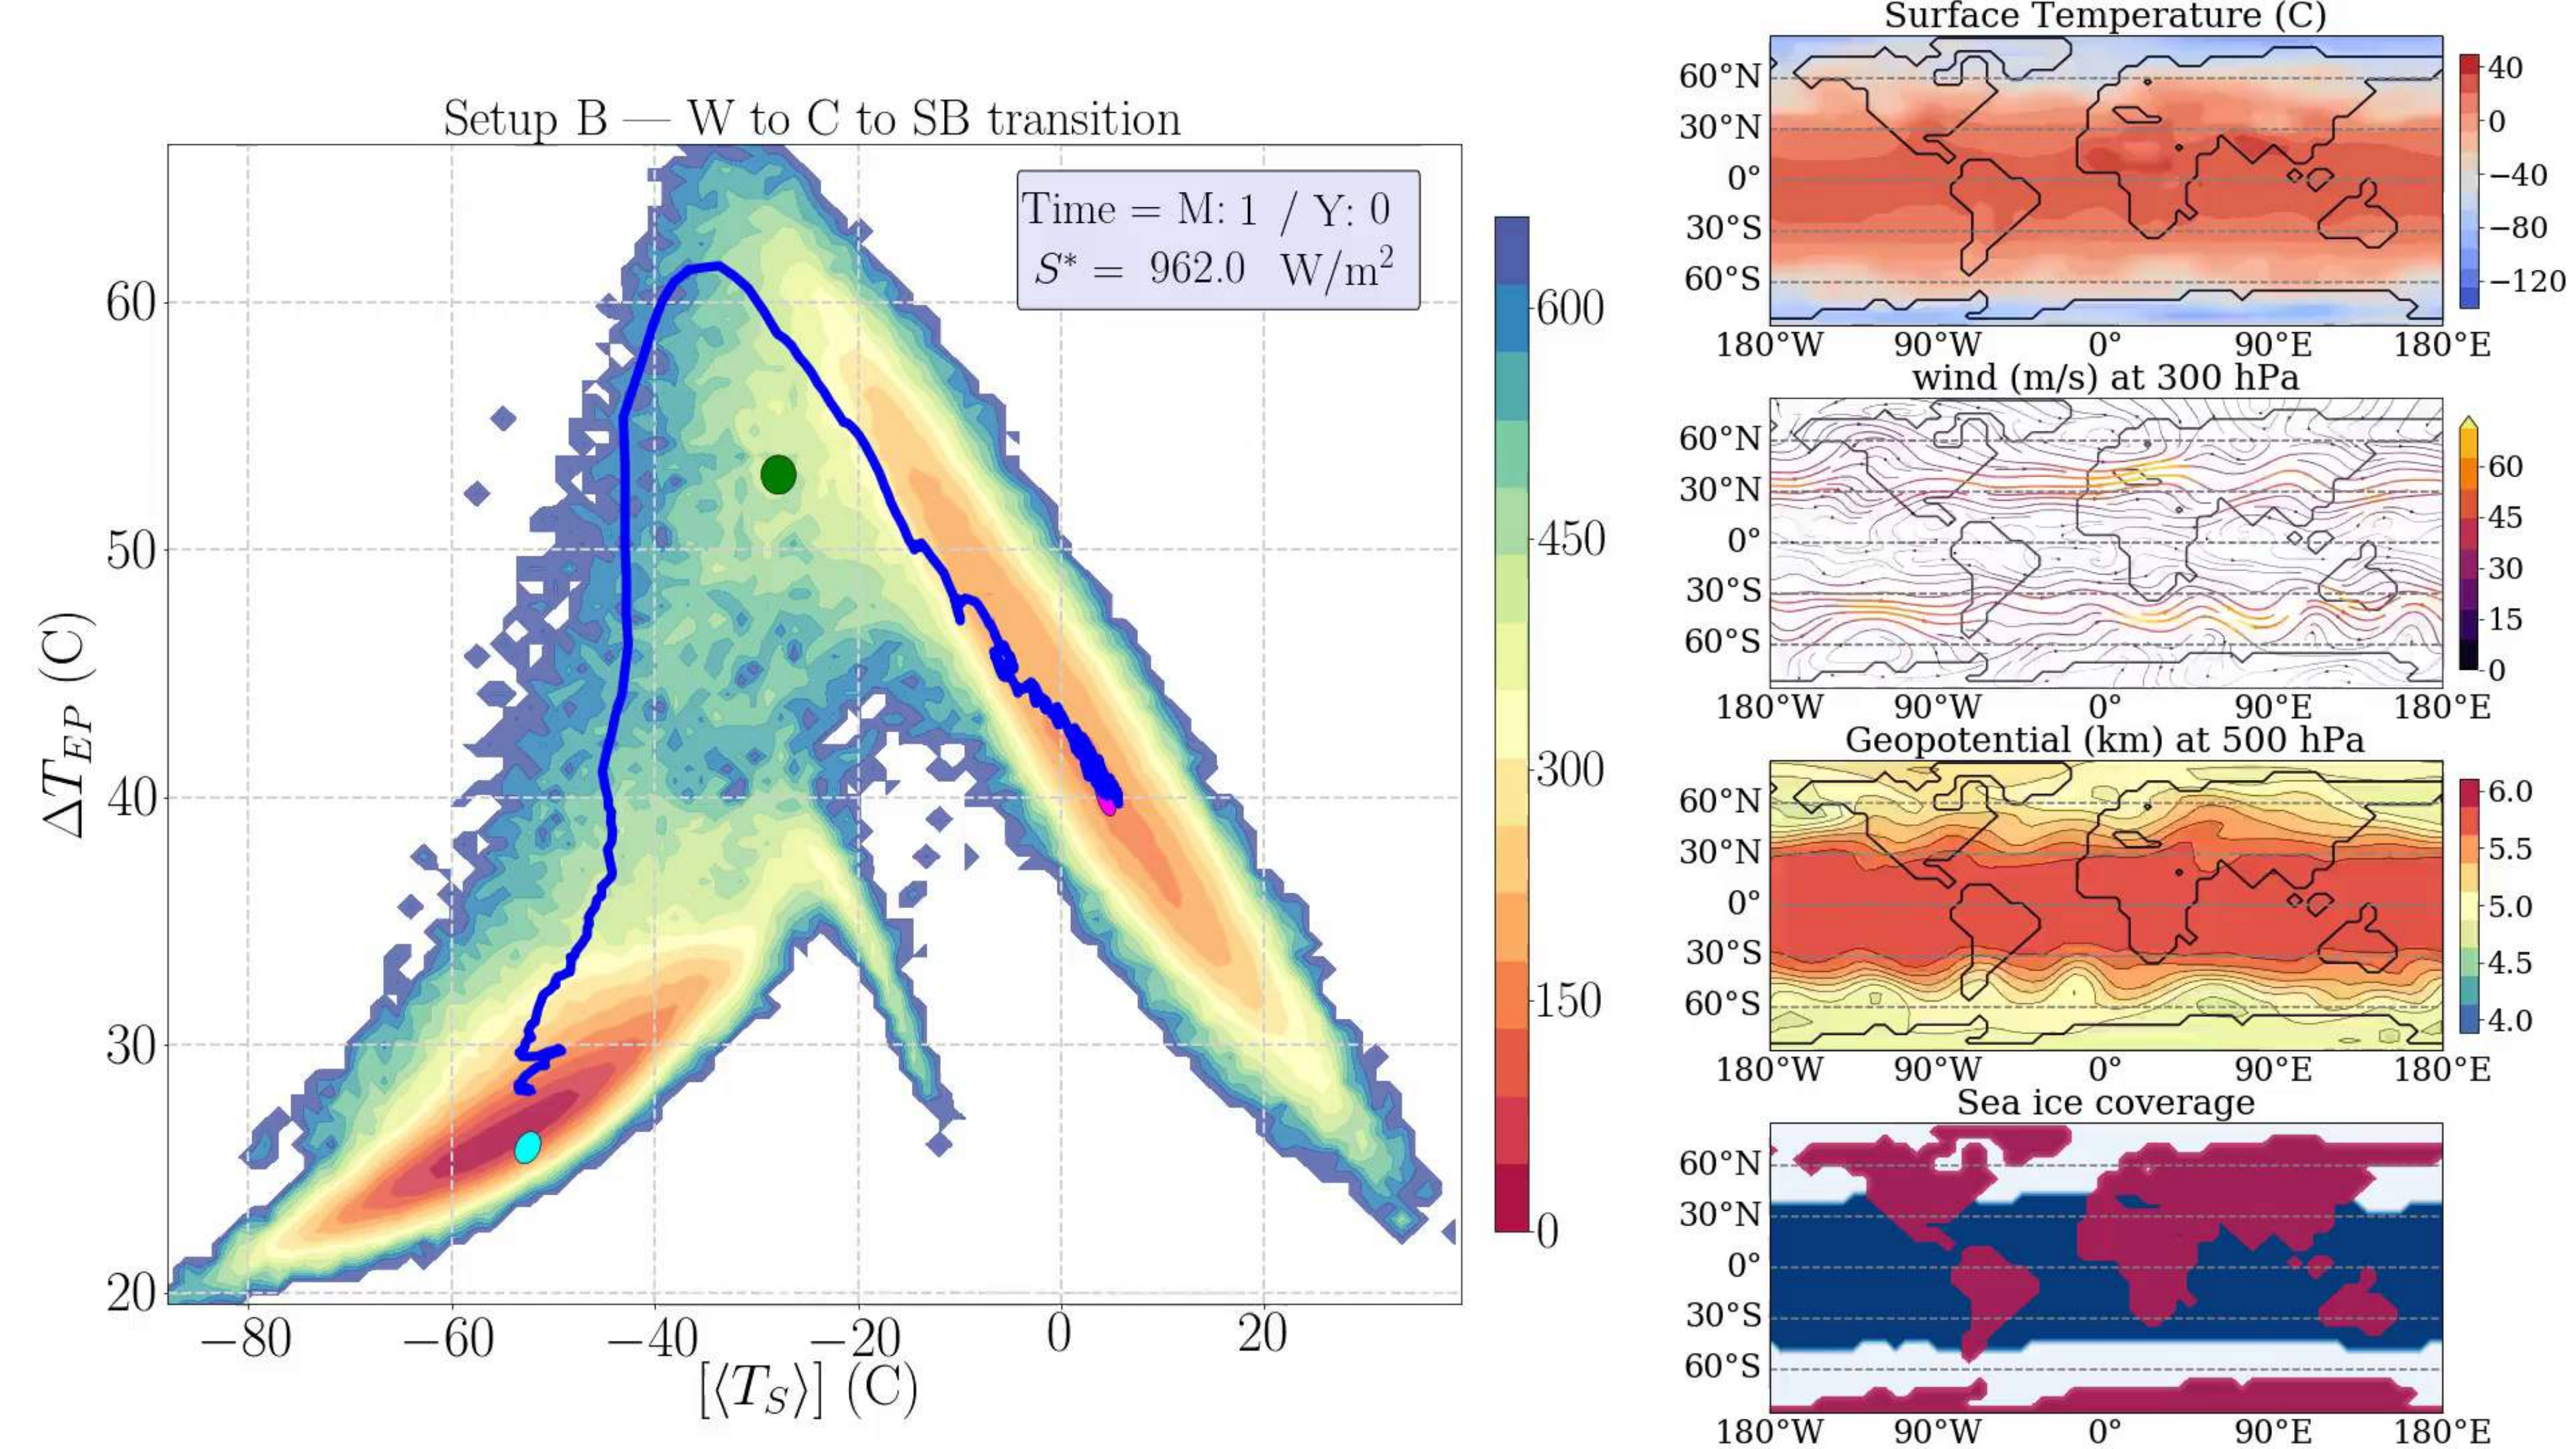}
	\caption{ Setup B: (left) Snowball to Cold to Warm transition. In this example the system starting from the SB basin of attraction spends a few years in the C basin of attraction before transitioning towards the W basin of attraction. This dataset is taken from $\sigma=12\%$ for setup B \cite{datapaper}. \href{https://youtu.be/0iFCrqUvhRg}{Click for video}. (right)  Warm to Cold to Snowball transition.  In this example the system starting from the W basin of attraction spends a few years in the C basin of attraction before transitioning towards the SB basin of attraction.  \href{https://youtu.be/6FuHZ-tB--A}{Click for video}}
	\label{fig:setup_B_SBCW} 
\end{figure}

\subsubsection{Noise induced transitions from C state}
In these animations we start from C state and then impose a much weaker noise, $\sigma = 6\%$ to perturb it and induce a transition towards either the W (Fig.~\ref{fig:setup_B_CW}-left) or the SB (Fig.~\ref{fig:setup_B_CW}-right) basin of attraction. The mean escape paths are included as a red (blue) line towards the W (SB) attractor.

\begin{figure}[!ht]
	\centering
	\includegraphics[width=0.49\linewidth]{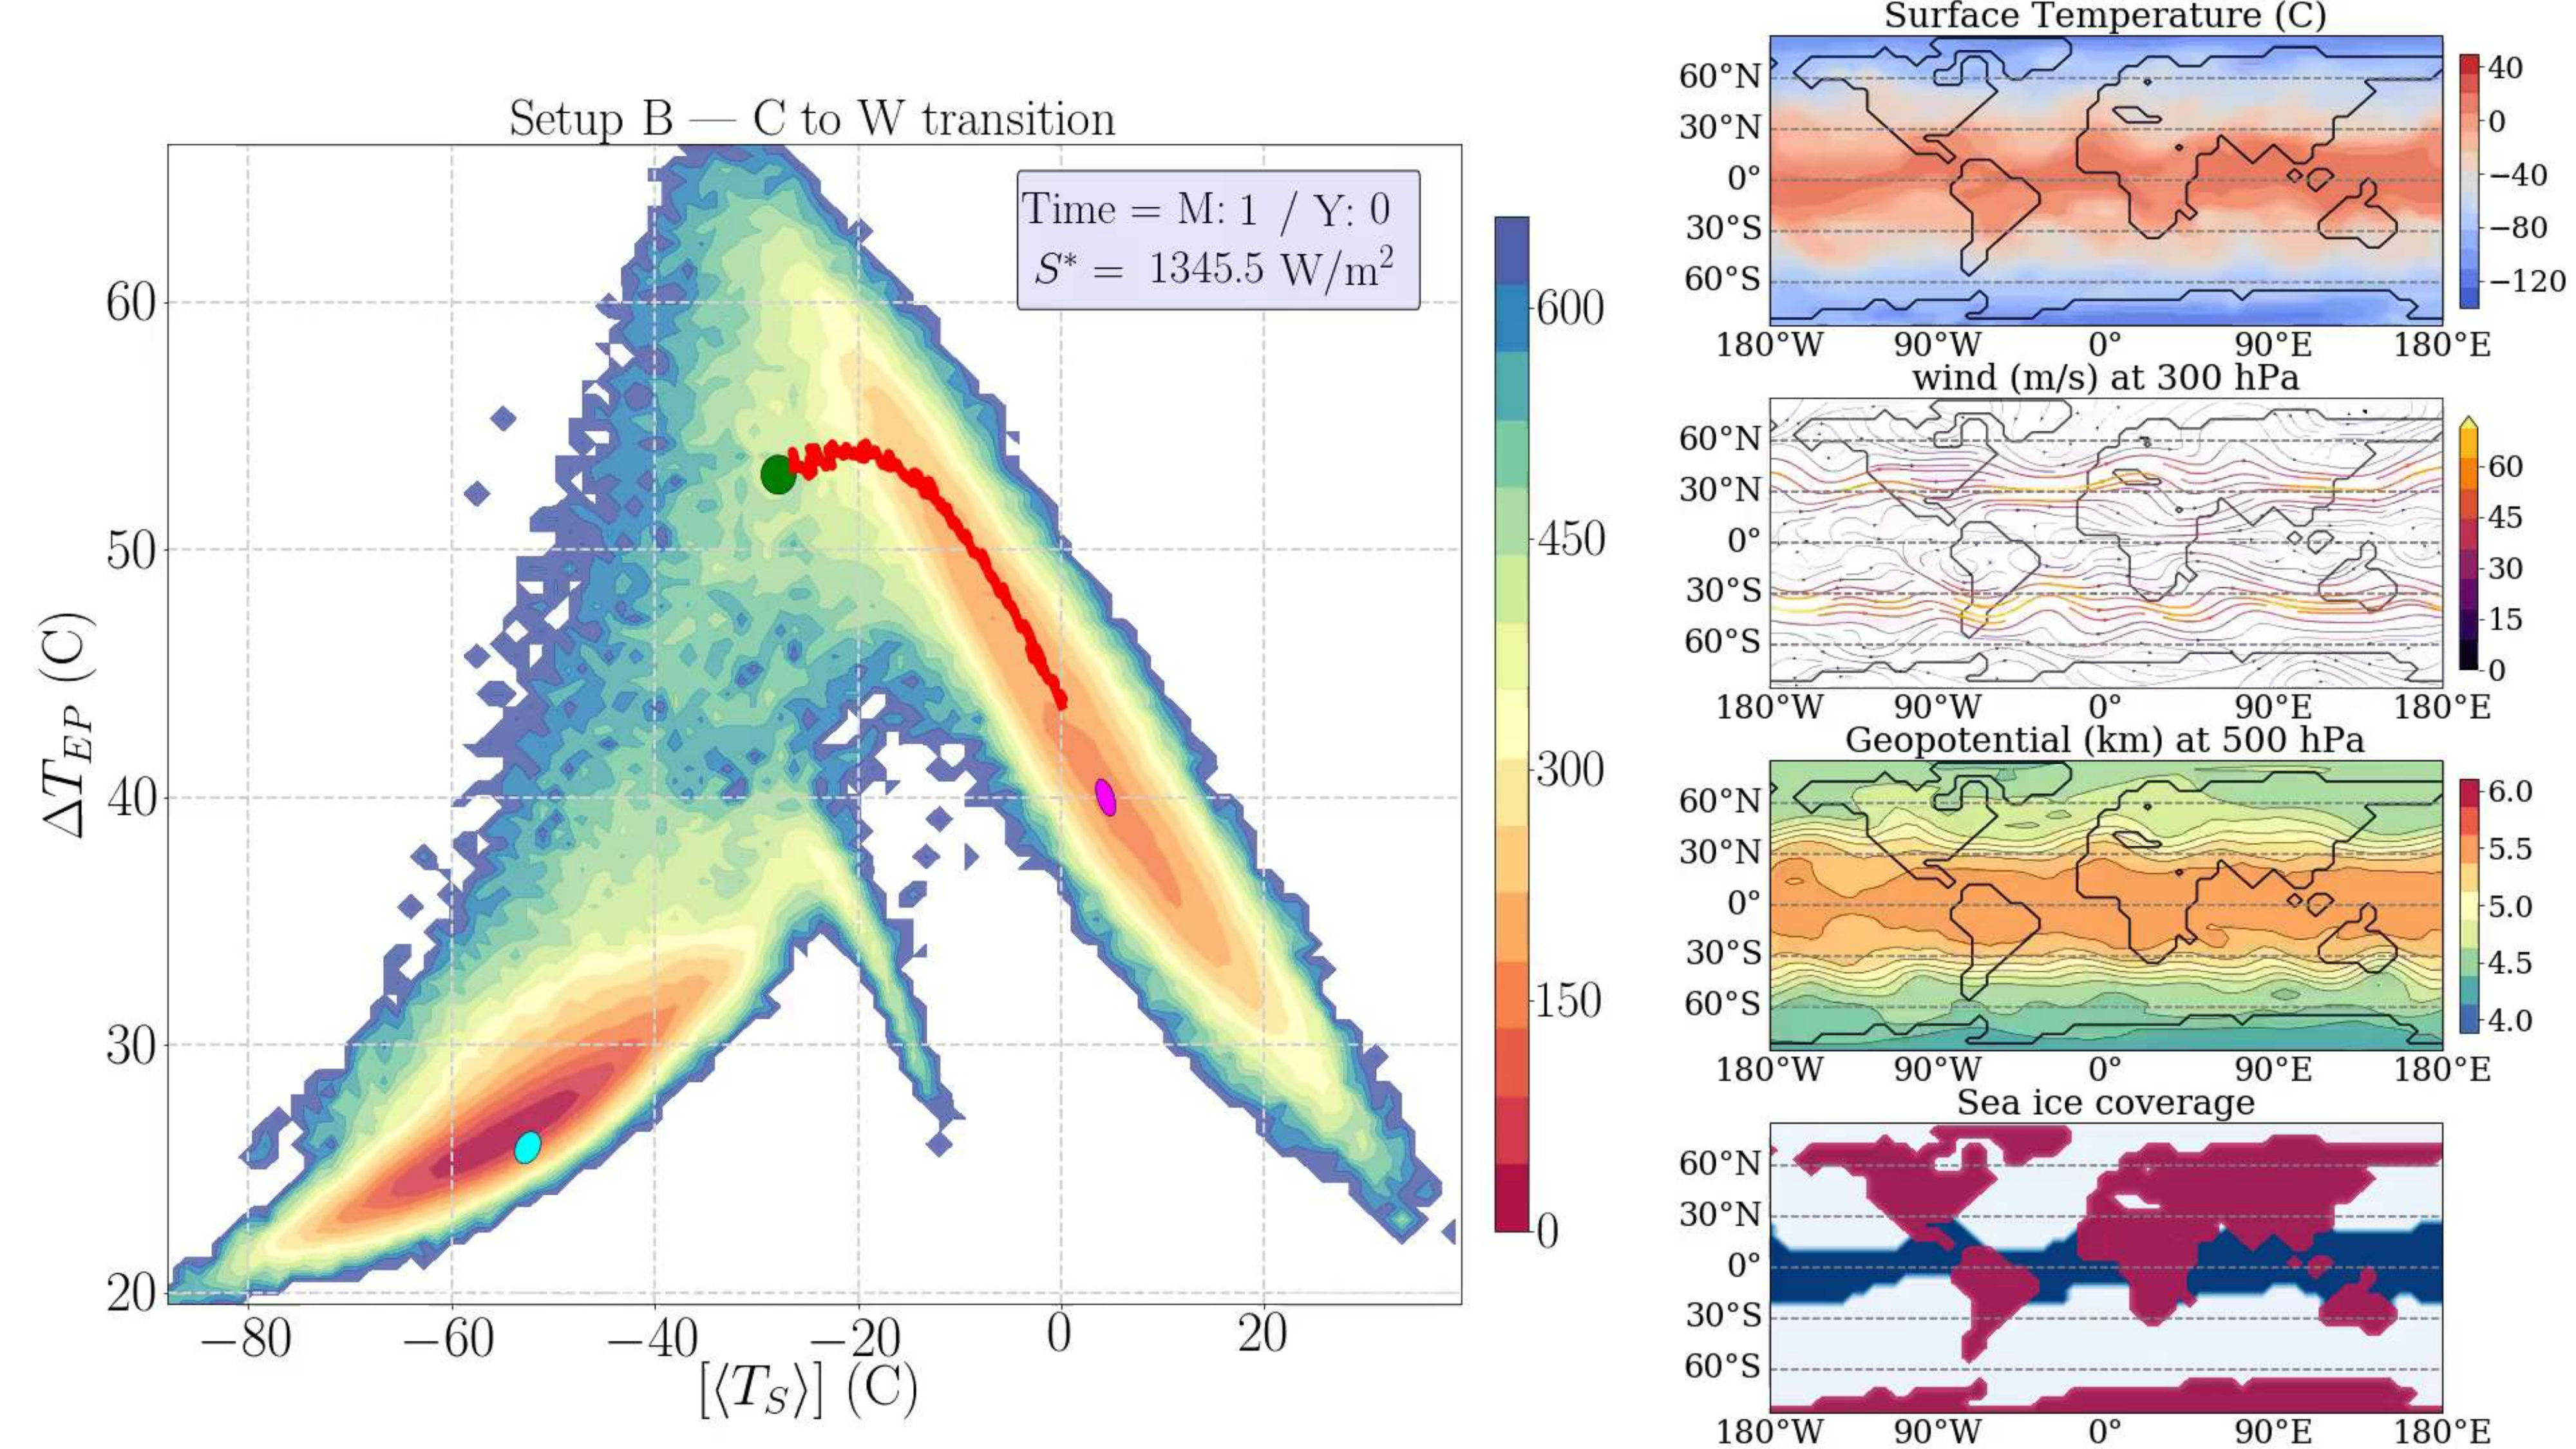}
	\includegraphics[width=0.49\linewidth]{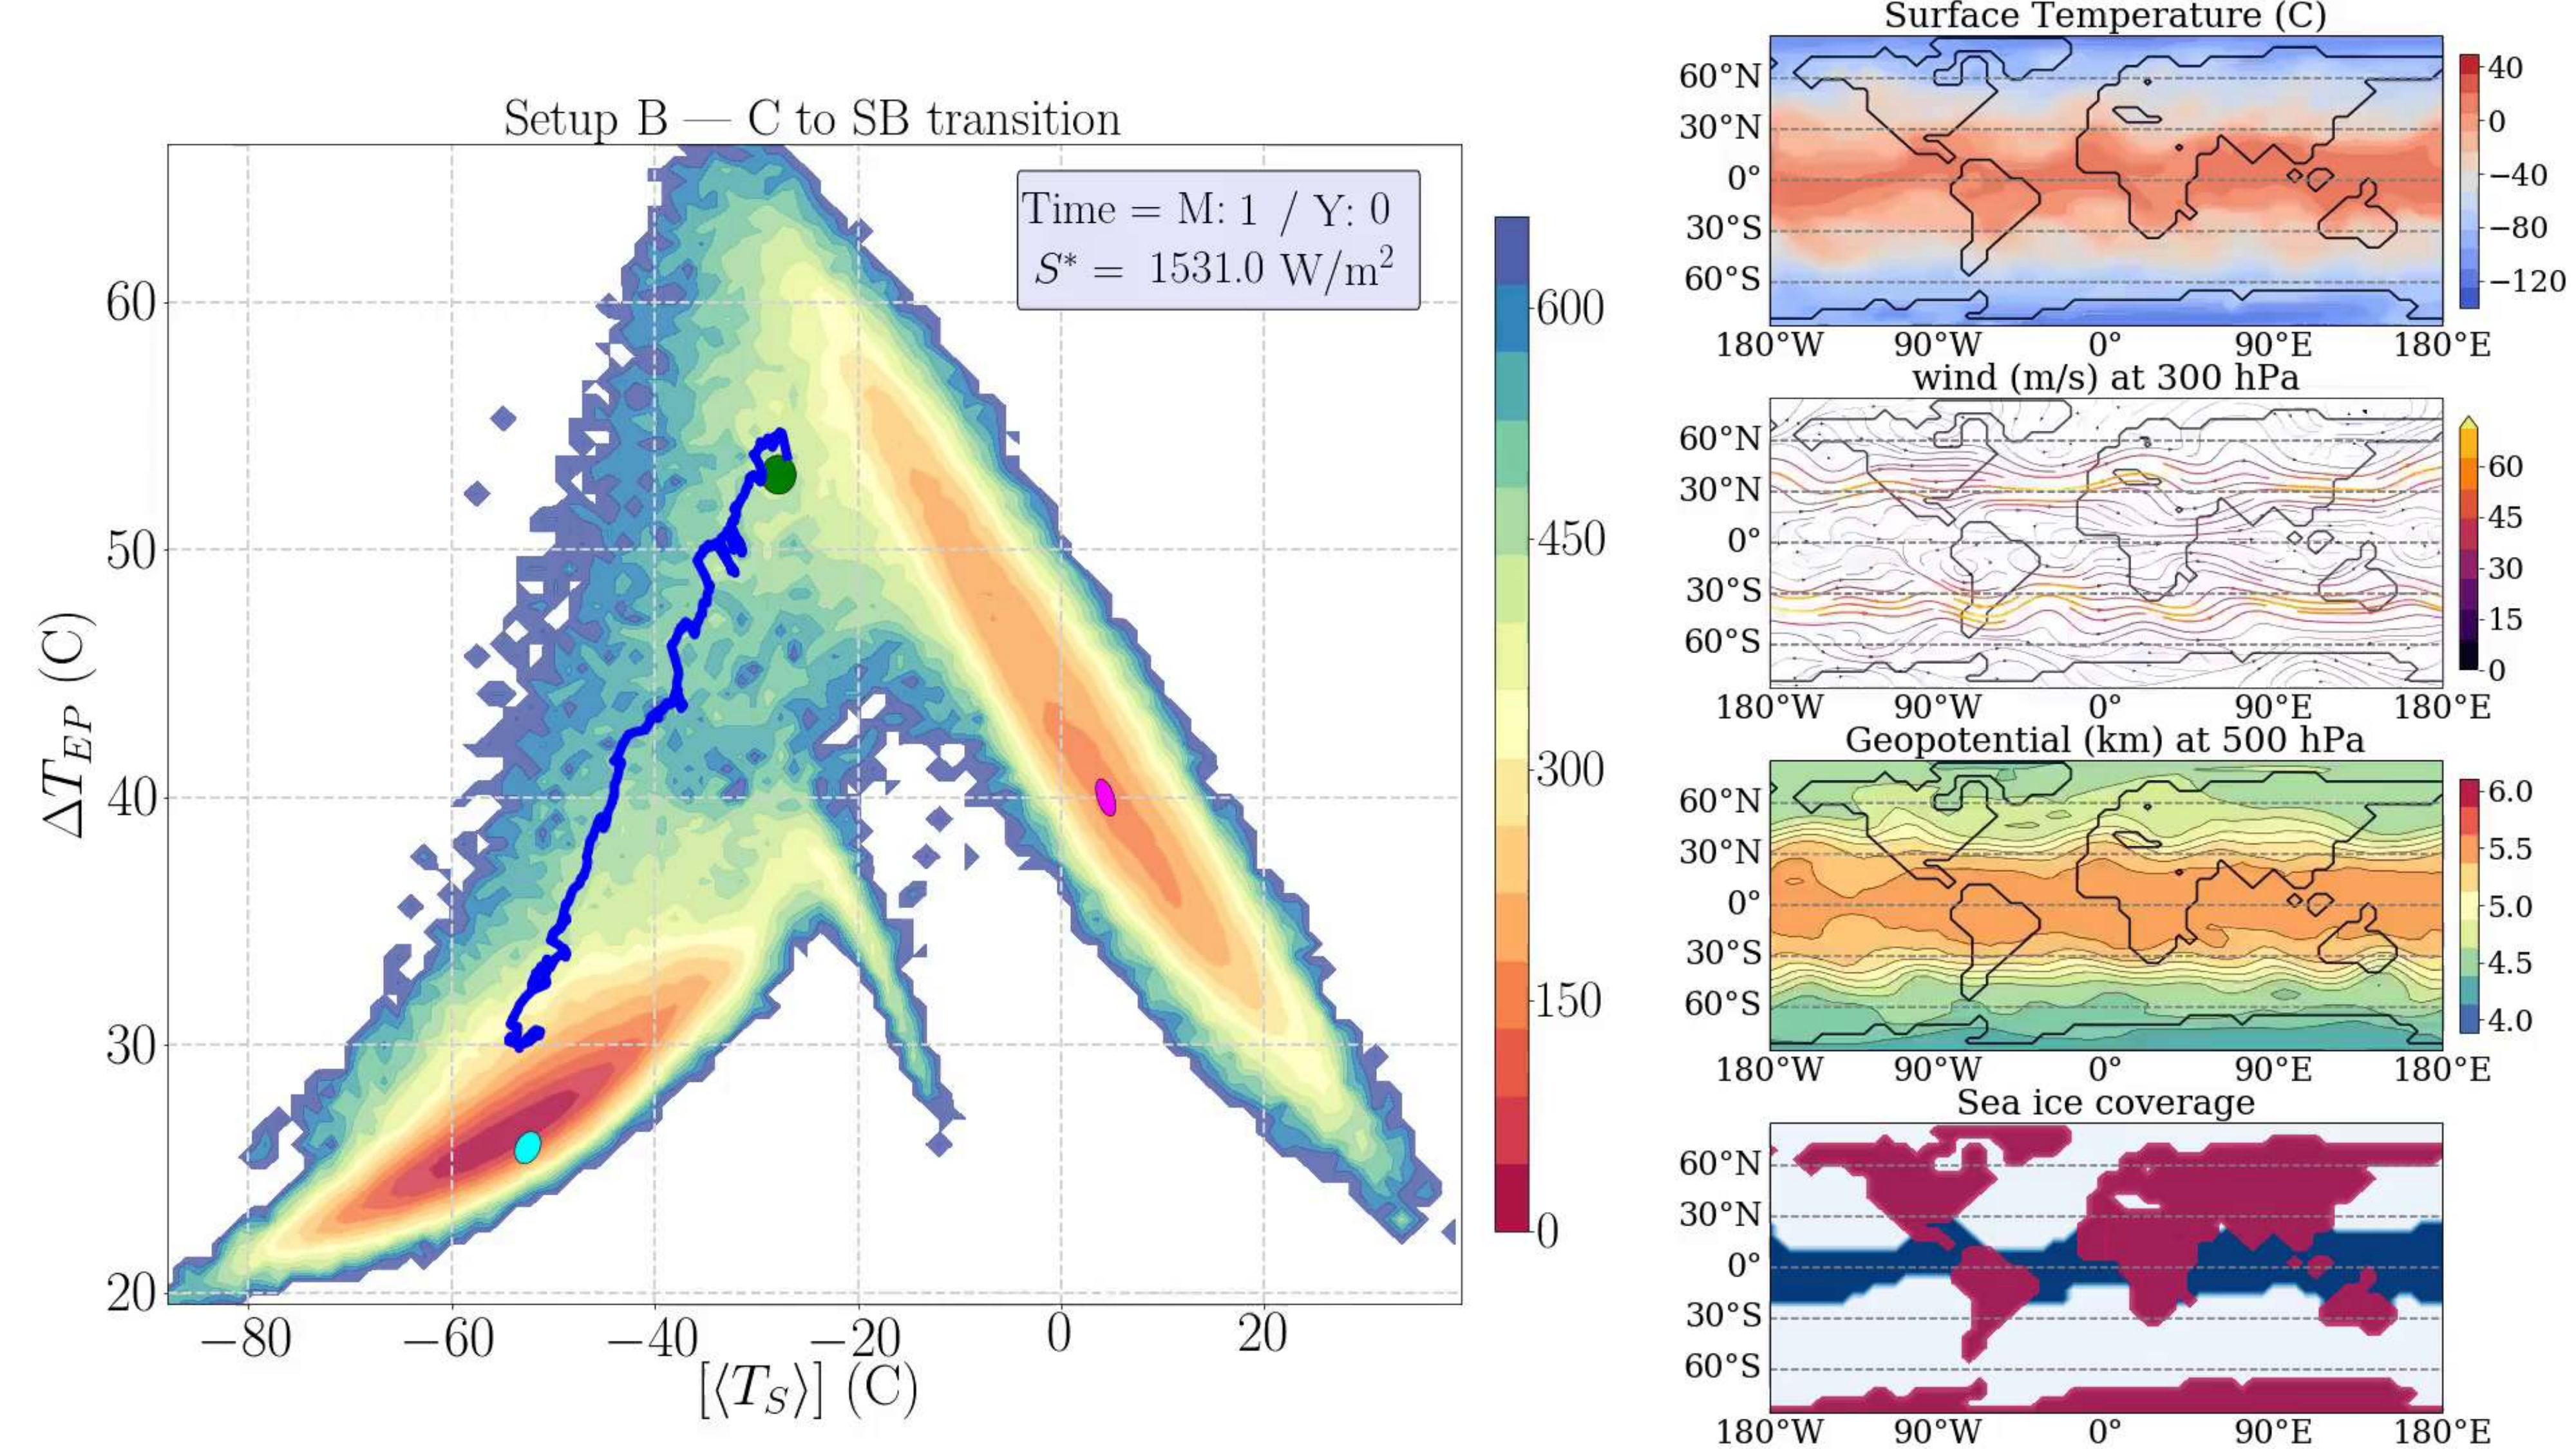}
	\caption{ Setup B: (left) Cold to Warm transition.   \href{https://youtu.be/Tc8TfQcAC5c}{Click for video}. (right) Cold to Snowball transition.   \href{https://youtu.be/-d23ksL0H0k}{Click for video}}
	\label{fig:setup_B_CW} 
\end{figure}

\subsubsection{Remark on the C state}

We would like to add a final remark regarding the numerical stability of the C state, as in a quite rare occasion, we observed a $C\rightarrow W$ transition with $\sigma=0$ of only one out of many relaxation trajectories, after evolving it for roughly 4000 years. Tracing back on the cause behind this, we identified a source of intrinsic noise in our model, related to the sea-ice module. In particular, we observed that, very rarely, certain oceanic grid points would abruptly ``flicker'' between presence or absence of sea-ice on a day-to-day basis. Note that PLASIM allows only a binary state for sea-ice, thus effectively introducing a truncation noise. Switching from sea-ice to open sea has dramatic consequences in the local energy budget, because the surface albedo goes from very high to very low. In some cases, such flickering would permanently change the status of nearby grid points, thus triggering a gradual long term elimination of the sea-ice coverage. Once a certain threshold was passed, a rapid transition to the W state was observed. The phenomenology of this numerical artifact indeed agrees with the very low $C\rightarrow W$ barrier we estimated.

\section{Transfer Operator and Finite State Markov Representation}\label{markovchain}
The transfer operator semigroup $\{\mathcal{L}^{t}\}_{t\geq 0}$ corresponding to the SDE given in Eq. (3) of the main text %~\ref{eqapp} 
can be defined as the solution of the Fokker-Planck Equation \cite{Risken1996}:
\begin{eqnarray}\label{fokkerplanck}
\partial _t\rho (\mathbf{x},t)&=\mathcal{A}\rho (\mathbf{x},t):=-\nabla \cdot \left(\mathbf{F}\rho(\mathbf{x},t) \right) \nonumber \\
&+ \frac{\sigma^2}{2}\sum _{i,j=1}^N\partial_{x_i,x_j} C(\mathbf{x})\rho (\mathbf{x},t).
\end{eqnarray}
where $\rho(\mathbf{x},t)=\mathcal{L}^t\rho _0(\mathbf{x})$ for some initial condition $\rho_0 \in L^1(X)$, and $\mathcal{L}^t=\exp\left(\mathcal{A} t\right)$. The transfer operator $\mathcal{L}^t$ describes the pushforward of an integrable function under the action of the dynamical system for a time duration of $t$. It turns out that $\mathcal{L}^t$ is a contraction and the set $\{ \mathcal{L}^t \}_{t\geq 0}$ is a $C_0$-semigroup, so that $\mathcal{L}^{t_1+t_2}=\mathcal{L}^{t_1}\mathcal{L}^{t_2}$ $\forall t_1,t_2\geq0$. The differential operator $\mathcal{A}$ is the generator of the $C_0$-semigroup.  The invariant measure is the  eigenvector with eigenvalue 0 of the operator $\mathcal{A}$: $\mathcal{A}\rho_\sigma(\mathbf{x})=0$ and can be normalised to one. The other eigenvectors of $\mathcal{A}$ integrate to zero and their corresponding eigenvalues have real part that is strictly smaller than zero if we assume that the system is mixing. The subdominant eigenvalue with largest real part controls the speed of convergence of an arbitrary initial measure to the invariant one.   

Typically, in many applications one needs to construct finite-state approximation of the phase space. We refer the reader to \cite{Tantet2018} for a detailed treatment of what follows below. To do this, we shall consider a finite shape-regular partition  phase-space $X$ into $M$ regions or \emph{boxes} $\{B_i\}_{i=1}^{M}$ and define $\mathbf{1}_{B_i}$ as the characteristic function on box $B_i \subset X$. Thus, we define the projection $P_M: L^1\left(X\right) \longrightarrow U_M : = \mathrm{Span}\left(\{\mathbf{1}_{B_i}\}_{i=1}^M \right)$ as
\begin{equation}
P_M f = \sum_{i=1}^M\mathbf{1}_{B_i}\frac{\langle f \mathbf{1}_{B_i} \rangle_{\rho_\sigma}} {\langle \mathbf{1}_{B_i} \rangle_{\rho_\sigma}}
\end{equation}
where $\langle g \rangle_{\rho_\sigma}= \int \rho_\sigma(\mathbf{x}) g(\mathbf{x}) \mathrm{d}\mathbf{x}$. It follows that the operator $P_M\mathcal{L}^t: U_M \longrightarrow U_N$ admits a matrix representation:
\begin{equation}\label{projected transfer operator}
\mathcal{M}^{t}_{i,j}:=\left(P_M\mathcal{L}^t\right)_{i,j}=\frac{\langle \mathbf{1}_{B_j} \mathcal{L}^t\mathbf{1}_{B_i} \rangle_{\rho_\sigma}}{\langle \mathbf{1}_{B_j} \rangle_{\rho_\sigma}},
\end{equation}
which happens to be a Markov or \emph{stochastic} matrix, so that $\sum _{j=1}^M\mathcal{M}_{i,j}=1$, $\mathcal{M}_{i,j}\geq 0$. The finite-state approximation to the invariant measure is obtained as $\lambda=1$ solution to the eigenvalue problem $\mathcal{M}\mathbf{u}=\lambda\mathbf{u}.$

%the number of basis functions required to resolve properly a given scale increases exponentially with the dimension. 

%The Ulam's conjecture says that if one one assumes that each side of the $N$-dimensional box $B_i$ scales with $h$ and If the invariant measure is smooth, as $h\rightarrow 0$, the corresponding sequence of finite-state invariant measures will converge to the actual invariant measure of the infinite dimensional operator. The construction of such a regular partition of the phase space is the basis of the so-called Ulam's method.

%High-dimensional systems, say of more than three dimensions, are not easily amenable to Ulam's method, since the number of basis functions required to resolve properly a given scale increases exponentially with the dimension. 

For high-dimensional systems -- say with $N\gg 3$ -- one is led to study the evolution of densities in a reduced space (the two-dimensional space  $([\langle T_S \rangle ],\Delta T_{EP})$ in the examples above). The procedure we follow goes  through the following steps: 1) we discretize  the transfer reduced operator on a finite family of basis functions in the projected space; 2) we estimate the transition probabilities in a frequentist way from a long time series. Unfortunately, the dynamics in the reduced space is non-Markovian, as clarified by the classical results by Mori and Zwanzig. As a result, the semigroup property of the transfer operator is in general lost for the projected operator:
%\begin{equation}\label{nonmarkov}
$\mathcal{M}^{t_1+t_2}_{i,j}=\left(P_M\left(\mathcal{L}^{t_1+t_2}\right)\right)_{i,j}=\left(P_M\left(\mathcal{L}^{t_1}\mathcal{L}^{t_2}\right)\right)_{i,j}\neq \left(P_M\left(\mathcal{L}^{t_1}\right)\right)_{i,k}\left(P_M\left(\mathcal{L}^{t_2}\right)\right)_{k,j}$, and the identification of the first subdominant eigenvectors and eigenvalues of $\mathcal{M^\tau}$ with the slowest decaying modes and their decay over a time scale of $\tau$ is only tentative. Nonetheless, by making a reasonable choice of $\tau$ and by considering observables that have a relevant projection on the reaction coordinates of the system and given an important contribution to the slow dynamical processes (in our case the ice-albedo and the radiative feedback and the large scale energy transports), one expects to find results that have at least qualitative relevance, as shown in Figs. 6 and 12 of the main text.% ~\ref{fig:ocdiff_0_sub} and Fig.~\ref{fig:ocdiff_1_sub} .

\section{Remark on the intrinsic dimension}
We include here a further supporting remark on the estimation of the intrinsic dimension (ID) of the manifold containing the data. It follows the approach described in \cite{faccoID}, where the number of points in abscissas is selected at random. In Fig.~\ref{fig:ID} the error bars are the standard deviation of the ID estimated over different samples of the same size. 
\begin{figure}[!ht]
	\centering
	\includegraphics[width=0.6\linewidth]{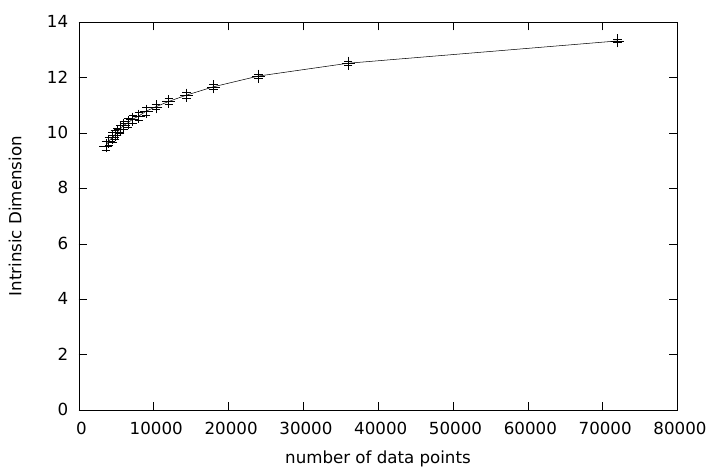}
	\caption{ The intrinsic dimension estimated for the data set analyzed in Fig 12, a trajectory of setup B and  $\sigma=12\%$  in the coordinate space of the temperatures at three different pressures (300, 500 and 1000 hPa) at 32  latitudes between -86$^o$ and 86 $^o$ (a total of 96 variables). }
	\label{fig:ID} 
\end{figure}

\section{Data Availability}
We provide the  data required to generate the figures of the main paper via a CC BY 4.0 license in \href{https://doi.org/10.6084/m9.figshare.13079489}{link} \cite{datapaper}. Within these files further instructions and information is given to allow the interested reader to either directly reproduce the figures, or others are the raw data one needs to reproduce the figures using the methodologies described in the paper. {\color{black}The videos are publicly available on the \texttt{youtube.com} platform through the provided links and can be freely downloaded from there.}

\bibliographystyle{RS}

\vskip2pc

\end{document}
